# Supplementary material for: Is Cross-Validation the Gold Standard to Evaluate Model Performance?
Source: arXiv:2407.02754 source file (2024-08-20)
Supplement: Supplementary file 1 [file appendix.tex]

\section{Related Work}\label{sec:work}
% =======
% %\paragraph{Organization.} In the following, we first review some evaluation criterion appeared in statistical learning and operations models in \Cref{sec:work}. Then we motivate our setup in \Cref{sec:pre} and our main results in \Cref{sec:main}. We concretize different data-driven models in \Cref{subsec:ierm}, \ref{subsec:reg} and \ref{subsec:parametric} respectively. We extend our method for nonsmooth objectives in \Cref{subsec:nonsmooth} and under the framework of contextual optimization approach in \Cref{subsec:context}. Finally, we present numerical studies on both synthetic and real data to demonstrate the usage of our approaches in \Cref{sec:numerical}.
% >>>>>>> f334df58b5d523ae2bfb130a45aedd2b3f37b770

\paragraph{Variations of Data-Driven Decision Models.} We mention several representative lines of works in view of \Cref{asp:represent} for $\paranx$ here.
%Examples include settings where the decision $x^*(\theta)$ is the output of a neural network with parameter vector $\theta$. $\theta$ can also be the parameters of a family of distributions $\{\P_{\theta},\theta \in \Theta\}$ and $\paranx$ is the corresponding decision under such parametrized distribution $\P_{\theta}$. 
Different model parametrization results in different decision rules. 
% the standard protocol of data-driven optimization is divided into two
% stages, i.e. first estimate the uncertainty parameter in the objective,
% optimize the cost in terms of the given model. The classical
Even with the same parametrization $\paranx$, the approach to estimate $\hat{\theta}$ 
%function mapping from parameter $\theta$ to decision $x$ 
can be different, especially when $\theta$ is the parameter of a family of distributions.
%even fixing the parameter within a space of distributions, the mapping from parameter to decisions can be different. 
The classical approach is the two-stage approach where one uses data to estimate 
% is first estimate
the % model
parameter $\hat{\theta}$, % i.e. from the unknown distribution,
and then obtains $\datax$ by optimizing under the estimated parametric distribution, i.e. $\E_{\P_{\hat{\theta}}}[h(x;\xi)]$~\citep{bertsimas2020predictive,hu2022fast}.  % from the observed data
% On one hand, to encode the parametric uncertainty from limited data
% directly into the
A more recent approach combines the parameter estimation and decision
making in an end-to-end
manner~\citep{donti2017task,agrawal2019differentiable}. For example, one can directly optimize over the objective $\frac{1}{n}\sum_{i = 1}^n h(\paranx;\xi_i)$ to attain $\hat{\theta}$ and associated $\datax$.
% optimization task efficiently, people suggests various approaches
% indicating that downstream aware approaches
Such approaches also go by 
operational statistics~\citep{liyanage2005practical} and
smart-predict-then-optimize~\citep{elmachtoub2022smart}. Furthermore, optimization problems often amplify errors in the parameter
estimate, and there are different approaches that attempt to mitigate this
phenomenon. 
These include 
% On the other hand, to reduce the problem with limited data, 
distributionally robust
optimization (DRO)~\citep{blanchet2019quantifying,duchi2019variance,gao2022distributionally}
and other regularization
approaches~\citep{maurer2009empirical,srivastava2021data}. 

\paragraph{Model Evaluation in Statistical and ML Practice.} Empirical
Risk Minimization (ERM) % in the supervised learning problem can be seen as
% a special type of
is, perhaps, the best known
approach % n the
for
data-driven optimization, and % estimation
% of its true performance has been considered over several decades.
several different methods have been proposed for estimating the true performance of the ERM
solution.  These include 
% Famous
% metrics including
AIC~\citep{akaike1974new}, Stein's unbiased risk
estimator (SURE)~\citep{stein1981estimation}, covariance
penalty~\citep{efron1986biased} % are developed to correct specific model
% bias for
that all correct the bias for 
particular cost functions and model
classes~\citep{anderson2004model}. %The notion of model bias induced in
% the model 
% to understand the complexity across different
% models.  
More recently, % researchers have extended the bias to more involved
% models such as the neural network design and
% understanding bias from these models.
these techniques have been extended to neural network models. 
\cite{murata1994network} applied network information criterion to select
the optimal network model. \cite{koh2017understanding} examined various
empirical optimization approaches from the influence function perspective
to understand how each point can affect overall model prediction
performance. \cite{novak2018sensitivity} found the bias is related to the
norm of input-output Jacobian of the network empirically. All of these terms capture a subset of problem instances and cannot incorporate general procedures.

%On the other hand, % there are some 

%estimators with one-shot optimization oracle by approximating LOOCV statistically offered computational benefits and enlightened the model selection and tuning 
%A survey of cross validation steps in model selection literature can be found in 
%The connections between two streams are provided in \cite{efron2004estimation}. 
%neural network
\paragraph{Model Comparison in Stochastic Optimization.}
\cite{lam2021impossibility} and
\cite{elmachtoub2023estimatethenoptimize}  % When generalizing
compare
% to
%model evaluation and selection % in
%to
data-driven optimization approaches in terms of
optimality gap, or equivalently excess risk or regret. %-- beyond 
% instead of
% just
% risk functions. % These works
Specifically, the comparison is based on an asymptotic generalization of the notion of stochastic
dominance.
% They
% compare a % subset
% set 
% of models under
% different scenarios and point out which method to prefer for a fixed
% parametric class asymptotically through the notion of stochastic
% dominance. 
Moreover, in contextual linear optimization, \cite{hu2022fast} compare the end-to-end and estimate-then-optimize procedures through the lens of  finite-sample generalization error bounds given certain marginal conditions. The compared approaches in these works constitute a subset of
decision classes than ours. More importantly,
the goal of our paper is not to identify the preference order of different decision classes for specific cost functions and samples through theoretical analysis but to remove the optimistic bias and accurately evaluate the true performance of each decision class practically.

 % given finite samples
%\hl{The preceding paragraph is very unclear. modified I was not able to edit it any further. TW: not sure if proper to put here, can we move it to Appendix or discussion parts?}

\paragraph{Other Debiasing Approaches in Operations.} Restricting to specific operations models, some specific types of model evaluation approaches are discussed in portfolio optimization~\citep{siegel2007performance} and newsvendor problem~\citep{siegel2021profit}. However, these approaches build on the assumption that the true distribution is well-specified within some parametric distribution classes, while our results do not require such a well-specification assumption.

In the data-driven optimization literature, when the objective is linear in the decision variable,
%e.g. $h(x;\xi) = \xi^{\top} g(x)$,  
\cite{ito2018unbiased,gupta2021small,gupta2022debiasing} remove the bias of linear optimization through Stein's lemma or sensitivity analysis. Compared to our work, their approaches are based on special structures in the linear optimization, where the estimated uncertainty from data $\Dscr^n$ and decisions are decoupled. As such, their problems do not suit any of our experimental instances in this paper. Moreover, some of these proposed methods require solving additional optimization problems and thus may not be computationally efficient. 

\section{Missing Discussion and Proofs in~\Cref{sec:main}}
\subsection{Discussion and Proof of~\Cref{thm:main}}
Before going to the main proof, we present the following technical lemma:
\begin{lemma}\label{lemma:matrix-expectation}
If $x \in \R^d$ is a random vector, $A \in \R^{d\times d}$ is a deterministic matrix, then $\E[x^{\top}A x] = \text{Tr}[AC]$, where $C = \E[x x^{\top}]$. 
\end{lemma}

\paragraph{Typical Conditions Satisfying Assumptions~\ref{asp:func} and~\ref{asp:represent}.} We divide some sufficient conditions by different optimization problem instances.

i) \underline{When $\paranx$ is expressed as some explicit analytic function of $\theta$ (empirical and variants of E2E)}, we can directly check whether \Cref{asp:represent} holds. In order for \Cref{asp:func} to hold, the sufficient condition is that $h(x;\xi)$ is twice differentiable with respect to $x$.

%In fact, throughout the whole analysis, due to Taylor expansion, we only need $h(\paranx;\xi)$ is twice continuous differentiable around $\theta^*$.

ii) \underline{When $\paranx$ is not an explicitly analytic function of $\theta$, such as an implicit function (ETO)}, more specifically, first-order condition (\Cref{asp:pf-fit-optimal}) holds, i.e. $\nabla_{x}\E_{\P_{\theta}}[h(x;\xi)] = 0$. Denote that first order condition to be of $f(\theta;\paranx) = 0$. 
%in terms of the relationship between the estimated parameter $\theta$ and the solution $\paranx$. 
In this case, in order for \Cref{asp:represent} to hold, one sufficient condition is that $f(\theta;x)$ is twice continuous differentiable in terms of $\theta$ and $x$ and $\nabla_{x}f(\theta;x) \neq 0$ (by implicit function theorem).
%and chain rule. 
In order for \Cref{asp:func} to hold, the sufficient condition is that $h(x;\xi)$ is twice differentiable with respect to $x$.

Below, we explicitly show how these gradients and hessians are computed by chain rule in practice.

If $\paranx$ is a scale, then the term we are interested in can be expressed by:
    \[\frac{\partial^2 h(x(\theta);\xi)}{\partial \theta^2} = \frac{\partial^2 h(x;\xi)}{\partial x^2}\frac{\partial x}{\partial \theta}\cdot \Para{\frac{\partial x}{\partial \theta}}^{\top} + \frac{\partial h(x;\xi)}{\partial x}\frac{\partial^2 x}{\partial \theta^2}.\]
    
When we are in case (i) above, all the terms can be computed exactly. To abbreviate notations here, we define $f_{x\theta} = \nabla_x \nabla_{\theta}f(\theta;x), f_{\theta} = \nabla_{\theta}f(\theta;x)$ and $f_{x} = \nabla_x f(\theta;x)$. Applying the standard implicit function theorem to any $i$-th component of $x$ and by chain rule, we would have:
\begin{align*}
    \frac{\partial x}{\partial \theta} & = - \frac{f_{\theta}}{f_x} \in \R^{D_{\theta}},\\
   \frac{\partial^2 x}{\partial \theta^2} &= \frac{-f_x^2 f_{\theta \theta} + f_x (f_{\theta}f_{x\theta} + f_{\theta x}f_{\theta}^{\top}) - f_{xx} f_{\theta}f_{\theta}^{\top}}{f_{x}^3} \in \R^{D_{\theta}\times D_{\theta}}.
\end{align*}
where $f_{x\theta}\in \R^{1\times D_{\theta}}, f_{\theta}\in \R^{D_{\theta}}, f_{\theta x} \in \R^{D_{\theta}\times 1}$. 
    
In general when $\paranx$ is a vector, we can apply the first-order condition $f(\hat{\theta};\datax) = 0$ with all $D_x$-th components of $\bm x = (x_1, \ldots, x_{D_x})^{\top}$ such that:
\begin{align*}
\frac{\partial h(\bm x(\theta);\xi)}{\partial \theta} &=    \sum_{i = 1}^{D_x}\frac{\partial h(\bm x;\xi)}{\partial x_i} \frac{\partial x_i}{\partial \theta},\\
\frac{\partial^2 h(\bm x(\theta);\xi)}{\partial \theta^2} &= \sum_{i = 1}^{D_x}\Para{\frac{\partial^2 h(\bm x;\xi)}{\partial x_i^2}\frac{\partial x_i}{\partial \theta}\cdot \Para{\frac{\partial x_i}{\partial \theta}}^{\top} + \frac{\partial h(\bm x;\xi)}{\partial x_i}\frac{\partial^2 x_i}{\partial \theta^2}} + 2\sum_{i = 1}^{D_x}\sum_{j \neq i}\frac{\partial^2 h(\bm x(\theta);\xi)}{\partial x_i \partial x_j} \frac{\partial x_i}{\partial \theta}\cdot\Para{\frac{\partial x_j}{\partial \theta}}^{\top}.
\end{align*}

In fact, although \Cref{asp:func} and \ref{asp:represent} are assumed for every $\theta$, in the theoretical proof we only require these conditions hold in a local sense that the twice differentiable condition holds around $\theta^*$. And these assumptions are set for every $\theta \in \Theta$ since we need to estimate $\gradp h(\datax;\xi)$ (and $\hessianp h(\datax;\xi)$) in practice where we need the differentiable condition holds for all $\theta \in \Theta$.

We now provide the proof of our main results. SLLN and WLLN stands for the Strong Law of Large Number (SLLN) and Weak Law of Large Number (WLLN) respectively.

\textit{Proof of~\Cref{thm:main}.}~In the following, if not specified for the subscript, $\E$ is taken under randomness of $\Dscr^n$ for the estimator $\hat{\theta}$ (including $\E_{\Dscr^n}, \E_{\hat{\theta}}$) and $\E_{\P^*}$ is taken under randomness of the random variable $\xi$. 

We introduce the following assumptions (to ensure the second moment exists through the proof) as a compliment formally here:
\begin{assumption}[Supplementary Assumptions]
$\E_{\P^*}[\nabla_{\theta} h(\bestx;\xi) \nabla_{\theta} h(\bestx;\xi)^{\top}] < \infty$ and $\E_{\P^*}[\hessianp h(\bestx;\xi)] < \infty$.
% \begin{itemize}
%     \item ;
%     % \item $\E_{\P^*}[\Para{\gradp h(\paranx;\xi)^{\top} IF_{\theta}(\xi)}^2] < \infty, \forall \theta \in \Theta$ (only required to bound $\text{Var}[\hat{A}_c] = O\Para{\frac{1}{n^2}}$. 
% \end{itemize}
\end{assumption}

%a simple approach would be applying Proposition 2 in \cite{gotoh2021calibration}.

We first want to show $\E[\hat{A}] = A + o\Para{\frac{1}{n}}$. And we divide the proof of this equation into three steps. 

\textbf{Step 1: Exposing the optimality gap.}~For any data-driven solution $\datax$, we can decompose the true evaluation $A(=\E_{\Dscr^n}\E_{\P^*}[h(\datax;\xi)])$ to be:
\begin{equation*}
    \begin{aligned}
        A &= A' + \E_{\P^*}[h(\bestx;\xi_i)] - \frac{1}{n}\sum_{i = 1}^n h(\bestx;\xi_i)\\
    \end{aligned}
\end{equation*}

where $A' = \E_{\Dscr^n}\E_{\P^*}[h(x^*(\hat{\theta});\xi) - h(x^*(\theta^*);\xi)] + \frac{1}{n}\sum_{i = 1}^n h(x^*(\theta^*);\xi_i)$. We see $\E[A] = \E[A']$ by:
\begin{equation}\label{eq:unbias-best}
    \E\Paran{\frac{1}{n}\sum_{i = 1}^n h(\bestx;\xi_i)} - \E_{\P^*}[h(\bestx;\xi)]  = \E_{\P^*}[h(\bestx;\xi)]  - \E_{\P^*}[h(\bestx;\xi)]  = 0.
\end{equation}
Therefore, in order to show $\hat{A}$ such that $\E[\hat{A}] = A + o\Para{\frac{1}{n}}$, it is equivalent to show that $\E[\hat{A} - A'] = o\Para{\frac{1}{n}}$. To compute the expectation of $A'$, we further decompose $A$:
\begin{equation}
    \begin{aligned}
        A' & = \frac{1}{n}\sum_{i = 1}^n h(x^*(\hat{\theta});\xi_i) + \underbrace{\frac{1}{n}\sum_{i = 1}^n h(x^*(\theta^*);\xi_i)  - \frac{1}{n}\sum_{i = 1}^n h(x^*(\hat{\theta});\xi_i)}_{T_1}\\
&+\underbrace{\E_{\Dscr^n}\E_{\P^*}[h(x^*(\hat{\theta});\xi) - h(x^*(\theta^*);\xi)]}_{T_2}\\
    \end{aligned}
\end{equation}

Intuitively, the terms $T_1$ and $T_2$ are due to the combination of optimism bias and estimation error under finite samples. We call them as the sample ``optimistic gap'' and true ``optimistic gap'' respectively. $T_1$ is random and $T_2$ is deterministic. Therefore, it is equivalent to show that: 
\[\E[T_1] + T_2 = \E[\hat{A}_c] + o\Para{\frac{1}{n}}.\]
 
\textbf{Step 2: Simplify the optimality gap here.}~We show that $\E[T_1 ] + T_2 = \E[\hat{A}_c'] + o\Para{\frac{1}{n}}$ for some approximated term $\hat{A}_c'$. 

For the term $T_1$, following Taylor expansion up to 2nd with Peano's Remainder at the center $\theta^*$ for the function $\frac{1}{n}\sum_{i = 1}^n h(\paranx;\xi_i)$ and~\Cref{asp:func}, we have:
\begin{equation}\label{eq:t1-expand}
    \begin{aligned}
        T_1 & = \frac{1}{n}\sum_{i = 1}^n \gradp h(\bestx;\xi_i)^{\top}(\theta^* - \hat{\theta}) - \frac{1}{2}(\theta^* - \hat{\theta})^{\top}\Para{\frac{1}{n}\sum_{i = 1}^n \hessianp h(\bestx;\xi_i)} (\theta^* - \hat{\theta}) + o\Para{\|\theta^* - \theta\|^2},
    \end{aligned}
\end{equation}
Then plugging the asymptotical expression of $\hat{\theta} - \theta^*$ in~\Cref{asp:theta-asymptotics} and take expectation over $T_1$ (noticing that $\E[\|\hat{\theta} - \theta^*\|^2] = O\Para{\frac{1}{n}}$), we obtain:
\begin{equation}\label{eq:oic-t1}
    \E[T_1] = \E\Paran{-\frac{1}{n}\sum_{i = 1}^n \nabla_{\theta} h(\bestx;\xi_i)^{\top}\Para{\frac{1}{n}\sum_{i = 1}^n IF_{\theta^*}(\xi_i) + \Delta}} - \frac{1}{2n}\text{Tr}[I_h(\theta^*)\Psi(\theta^*)] + o\Para{\frac{1}{n}},\\
\end{equation}
where $\underline{\Delta = \hat{\theta} - \theta^* - \frac{1}{n}\sum_{i = 1}^n IF_{\theta^*}(\xi_i)}$ to be the higher order term of the estimation error with $\E[\Delta \Delta^{\top}] = O\Para{\frac{1}{n}}$ from \Cref{asp:theta-asymptotics}. The second term of the right-hand side in \Cref{eq:oic-t1} follows by:
\begin{equation}\label{eq:second-order-asymp-theta}
\begin{aligned}
    &\quad \E\Paran{(\theta^* - \hat{\theta})^{\top}\E_{\hat{\P}_n}[\gradp h(\bestx;\xi)](\theta^* - \hat{\theta})}\\
    & = \E\Paran{(\theta^* - \hat{\theta})^{\top}\E_{\P^*}[\gradp h(\bestx;\xi)](\theta^* - \hat{\theta})} + o\Para{\frac{1}{n}} \\
    & = \frac{1}{n}\text{Tr}[I_h(\theta^*) \Psi(\theta^*)]+ o\Para{\frac{1}{n}},
\end{aligned}
\end{equation}
where the first equality is a combination result of $\E_{\hat{\P}_n}[\hessianp h(\bestx;\xi)] \overset{a.s.}{\to} \E_{\P^*}[\hessianp h(\bestx;\xi)]$ by SLLN and $\E[\|\hat{\theta} - \theta^*\|^2] = O\Para{\frac{1}{n}}$. The second equality above follows by observing $\E[(\hat{\theta} - \theta^*)(\hat{\theta} - \theta^*)^{\top}] = \frac{\Psi(\theta^*)}{n} + o\Para{\frac{1}{n}}$ as well as a result of~\Cref{lemma:matrix-expectation}. 
% Then we compare the difference between the left-hand side in~\Cref{eq:second-order-asymp-theta} and the second term in the right-hand side in~\Cref{eq:t1-expand} under expectation, i.e.:
% \begin{equation}
%     \begin{aligned}
%         & \E\Paran{(\theta^* - \hat{\theta})^{\top}\Para{\frac{1}{n}\sum_{i = 1}^n \hessianp h(\bestx;\xi_i) - \E_{\P^*}[\hessianp h(\bestx;\xi)]} (\theta^* - \hat{\theta})}\\
%         & = \E\Paran{(\theta^* - \hat{\theta})^{\top}\Para{\E_{\P_n}[\hessianp h(x^*(\tilde{\theta});\xi_i)] - \E_{\P_n}[\hessianp h(\bestx;\xi)]} (\theta^* - \hat{\theta})}  + o\Para{\frac{1}{n}}\\
%         & = o\Para{\frac{1}{n}} + o\Para{\frac{1}{n}} = o\Para{\frac{1}{n}},
%     \end{aligned}
% \end{equation}
% where the first equality follows by noticing $\E_{\P_n}[\hessianp h(\bestx;\xi)] = \E_{\P^*}[\hessianp h(\bestx;\xi)] + O_p\Para{\frac{1}{\sqrt{n}}}$ by central limit theorem. And the second equality follows by the definition of $\tilde{\theta} \convp \theta^*$ as $n \to \infty$, which implies~\Cref{eq:second-order-asymp-theta}.

Similarly in $T_2$, following the Taylor second order expansion at the center $\theta^*$, we have:
\begin{equation}\label{eq:t2-expand}
\begin{aligned}
    T_2 &= \E_{\P^*}[\nabla_{\theta}h(x^*(\theta^*);\xi)]^{\top}\E\Paran{\frac{1}{n}\sum_{i = 1}^n IF_{\theta^*}(\xi_i) + \Delta}+ \frac{1}{2n}\text{Tr}[I_h(\theta^*)\Psi(\theta^*)] + o\Para{\frac{1}{n}}\\
    & = \E_{\P^*}[\nabla_{\theta}h(x^*(\theta^*);\xi)]^{\top} \E_{\Dscr^n}[\Delta]+ \frac{1}{2n}\text{Tr}[I_h(\theta^*)\Psi(\theta^*)] + o\Para{\frac{1}{n}},
\end{aligned}
\end{equation}
where the second equality in \Cref{eq:t2-expand} follows by $\E[IF_{\theta^*}(\xi)] = 0$. Combining~\Cref{eq:oic-t1} and~\Cref{eq:t2-expand}, we have:
\begin{equation}\label{eq:t1-t2}
    \begin{aligned}
        \E[T_1] + T_2  & = \E\Paran{-\frac{1}{n}\sum_{i = 1}^n \nabla_{\theta} h(\bestx;\xi_i)^{\top}\frac{1}{n}\sum_{i = 1}^n IF_{\theta^*}(\xi_i)} -\E\Paran{\frac{1}{n}\sum_{i = 1}^n \nabla_{\theta} h(\bestx;\xi_i)^{\top} \Delta}\\ &\quad + \E_{\P^*}[\nabla_{\theta}h(x^*(\theta^*);\xi)]^{\top} \E_{\Dscr^n}[\Delta]\\
        & = -\E\Paran{\frac{1}{n}\sum_{i = 1}^n \nabla_{\theta} h(\bestx;\xi_i)^{\top}\frac{1}{n}\sum_{i = 1}^n IF_{\theta^*}(\xi_i)} + o\Para{\frac{1}{n}},
    \end{aligned}
\end{equation}
where the second equality in \Cref{eq:t1-t2} is from the following result (here we abbreviate $\underline{g(\xi_i) := \nabla_{\theta}h(x^*(\theta^*);\xi_i)}$ for simplicity):
\begin{equation}\label{eq:if2}
\begin{aligned}
    &\E_{\P^*}[\nabla_{\theta}h(x^*(\theta^*);\xi)]^{\top} \E_{\Dscr^n}[\Delta] - \E_{\Dscr^n}\Paran{\frac{1}{n}\sum_{i = 1}^n \nabla_{\theta} h(\bestx;\xi_i)^{\top} \Delta}\\
    =& \E_{\Dscr^n}\Para{\Paran{\E_{\P^*}[\nabla_{\theta}h(x^*(\theta^*);\xi)] - \E_{\hat{\P}_n}[\nabla_{\theta}h(x^*(\theta^*);\xi)]}^{\top}\Delta}\\
    \leq & \sqrt{\E_{\Dscr^n}[\|\E_{\P^*}[g(\xi)] - \E_{\hat{\P}_n}[g(\xi)]\|_2^2]}\sqrt{\E_{\Dscr^n}[\|\Delta\|_2^2]}\\
    = & O\Para{\frac{1}{\sqrt{n}}}\sqrt{ \E_{\Dscr^n}\Para{\text{Tr}[\Delta\Delta^{\top}]}} =o\Para{\frac{1}{n}}.
\end{aligned}
\end{equation}
where the first inequality in \Cref{eq:if2} follows by $\E[x^{\top}y] \leq \E[\|x\|_2\|y\|_2] \leq \sqrt{\E[\|x\|_2^2]}\sqrt{\E[\|y\|_2^2]}$. And the second inequality in \Cref{eq:if2} follows by observing the simple fact (MSE error of sample mean is $O\Para{\frac{1}{n}}$) that:
\[\E_{\Dscr^n}\Paran{\Para{\E_{\P^*}[g(\xi)] - \E_{\hat{\P}_n}[g(\xi)]}^2} = O\Para{\frac{1}{n}}\]
The last equality in \Cref{eq:if2} to bound $\text{Tr}[\Delta \Delta^{\top}]$ follows by $\E_{\Dscr^n}(\text{Tr}[\Delta \Delta^{\top}]) = \text{Tr}\Paran{\E_{\Dscr^n}[\Delta \Delta^{\top}]} = O\Para{\frac{1}{n}}$ from \Cref{asp:theta-asymptotics}.
%And the second inequality follows by:
%the first term $\|\E_{\P^*}[\nabla_{\theta}h(x^*(\theta^*);\xi)] - \E_{\hat{\P}_n}[\nabla_{\theta}h(x^*(\theta^*);\xi)]\|_{\infty}$ is bounded by Chebyshev inequality such that $\sqrt{\E_{\Dscr^n}[\|\E_{\P^*}[\nabla_{\theta}h(x^*(\theta^*);\xi)] - \E_{\hat{\P}_n}[\nabla_{\theta}h(x^*(\theta^*);\xi)]\|_{\infty}^2]} = O\Para{\frac{1}{\sqrt{n}}}$ while the second term is of order $O\Para{\frac{1}{n}}$ given by \Cref{asp:theta-asymptotics}. 
Therefore, the left-hand side of~\Cref{eq:if2} is bounded by $o\Para{\frac{1}{n}}$ and the second equality in \Cref{eq:t1-t2} holds.

Then back to the first term in right-hand side of~\Cref{eq:t1-t2}, i.e.:
\begin{equation}\label{eq:debias-term}
\begin{aligned}
    \E\Paran{\Para{\frac{1}{n}\sum_{i = 1}^n g(\xi_i)}^{\top}\frac{1}{n}\sum_{i = 1}^n IF_{\theta^*}(\xi_i)}& = \E\Paran{\frac{1}{n^2}\sum_{i = 1}^n g(\xi_i)^{\top} IF_{\theta^*}(\xi_i)} + \E\Paran{\frac{1}{n^2}\sum_{i = 1}^n \sum_{j \neq i} g(\xi_i)^{\top}IF_{\theta^*}(\xi_j)}\\
    & = \E\Paran{\frac{1}{n^2}\sum_{i = 1}^n g(\xi_i)^{\top} IF_{\theta^*}(\xi_i)} + \frac{1}{n^2}\sum_{i = 1}^n \sum_{j \neq i} \E[g(\xi_i)]^{\top}\E[IF_{\theta^*}(\xi_j)]\\
    & = \E\Paran{\frac{1}{n^2}\sum_{i = 1}^n g(\xi_i)^{\top} IF_{\theta^*}(\xi_i)} + 0,\\
\end{aligned}
\end{equation}
where the second inequality is based on the independence of $g(\xi_i)$ and $IF_{\theta^*}\xi_j)$ for $i \neq j$. And the third equality follows by $\E[IF_{\theta^*}(\xi)] = 0$ such that the second interaction term would be 0. 

Denote $\hat{A}_c' = -\frac{1}{n^2}\sum_{i= 1}^n \nabla_{\theta} h(\bestx;\xi_i)^{\top}IF_{\theta^*}(\xi_i)$, given that $\hat{A}_o = \frac{1}{n}\sum_{i = 1}^n h(\datax;\xi_i)$, comparing the two terms, the previous arguments already show that:
\[\E[\hat{A}_c' + \hat{A}_o] = \E[T_1] + T_2 + \E[\hat{A}_o] = A + o\Para{\frac{1}{n}}.\]

\textbf{Step 3: Controlling the estimation error between $\hat{A}_c$ and $\hat{A}_c'$.}~

Then to show $\E[T_1] + T_2 = \E[\hat{A}_c] + o\Para{\frac{1}{n}}$, we only need to illustrate:
\begin{equation}\label{eq:oic-unbiased0}
    (\E[\hat{A}_c' - \hat{A}_c] = )\E\Paran{\frac{1}{n^2}\sum_{i = 1}^n \Para{\nabla_{\theta} h(\bestx;\xi_i)^{\top} IF_{\theta^*}(\xi_i) - \nabla_{\theta} h(\datax;\xi_i)^{\top} \hat{IF}_{\hat{\theta}}(\xi_i)}} = o\Para{\frac{1}{n}}
\end{equation}
For now we can assume $\gradp h(\bestx;\xi), IF_{\theta^*}(\xi)$ to be scales instead of vectors since these are of finite dimensions and we are only interested the results up to $o\Para{\frac{1}{n}}$\footnote{This works in our setups, i.e. we are in a relative low-dimensional problem setup, i.e. $D_{\xi}/n = o(1)$}. If \Cref{eq:oic-unbiased0} holds for the scales, then left-hand side of \Cref{eq:oic-unbiased0} in the vector version would be $D_{\xi}\times o\Para{\frac{1}{n}} = o\Para{\frac{1}{n}}$ too. Therefore from properties of the expectation, to show \Cref{eq:oic-unbiased0}, it is equivalent to show the following thing:
\begin{equation}\label{eq:oic-unbiased1}
    \E_{\Dscr^n}\Paran{\gradp h(\bestx;\xi) IF_{\theta^*}(\xi) - \gradp h(\datax;\xi) \hat{IF}_{\hat{\theta}}(\xi)} = o(1), \forall \xi \in \{\xi_1, \ldots, \xi_n\}.
\end{equation}
We decompose the left-hand side of \Cref{eq:oic-unbiased1} as:
\begin{equation*}\label{eq:oic-unbiased2}
    \begin{aligned}
        &\quad\E_{\Dscr^n}\Paran{\gradp h(\datax;\xi) \hat{IF}_{\hat{\theta}}(\xi)} - \gradp h(\bestx;\xi) IF_{\theta^*}(\xi) \\
        & = \E_{\Dscr^n}\Paran{\gradp h(\datax;\xi) \Para{\hat{IF}_{\hat{\theta}}(\xi) - IF_{\theta^*}(\xi)}} + \E_{\Dscr^n}\Paran{\Para{\gradp h(\datax;\xi) - \gradp h(\bestx;\xi)}IF_{\theta^*}(\xi)} \\
        & + \E_{\Dscr^n}\Paran{\Para{\hat{IF}_{\hat{\theta}}(\xi) - IF_{\theta^*}(\xi)}\Para{\gradp h(\datax;\xi) - \gradp h(\bestx;\xi)}}\\
    \end{aligned}
\end{equation*}
Notice that $\E_{\Dscr^n}[(\hat{IF}_{\hat{\theta}}(\xi) - IF_{\theta^*}(\xi))^2] = o(1)$ from \Cref{asp:theta-asymptotics}. And from \Cref{asp:func} that $h(\paranx;\xi)$ is twice continuous differentiable,  we have:
\[\E_{\Dscr^n}[(\gradp h(\datax;\xi) - \gradp h(\bestx;\xi))^2] = \E_{\Dscr^n}[(O(|\hat{\theta} - \theta^*|))^2] = o\Para{\frac{1}{n}} = o(1).\]
Similarly, we can show $\E_{\Dscr^n}[(\gradp h(\datax;\xi))^2] = o(1)$. Then we can apply Cauchy-Schwartz inequality to each of three terms the right-hand side in \Cref{eq:oic-unbiased2} with the form $\E[xy]\leq \sqrt{\E[x^2]}\sqrt{\E[y^2]} = o(1)$ and obtain that each of these three terms is of the order $o(1)$. This replies that \Cref{eq:oic-unbiased0} holds and we finish the first part of the \Cref{thm:main} $\E[\hat{A}_c + \hat{A}_o] = A + o\Para{\frac{1}{n}}$.

% And the first term is based on the fact that $\hat{IF}_{\hat{\theta}}(\xi) = IF_{\theta^*}(\xi) + o_p(1)$ from~\Cref{asp:theta-asymptotics}, $\nabla_{\theta}h(x^*(\hat{\theta});\xi_i) = \nabla_{\theta}h(x^*(\theta^*);\xi_i) + o_p(1) = g(\xi_i) + o_p(1)$, which matches the definition of $\hat{A}_c$. Therefore, we obtain the expression of $\hat{A}_o$ and $\hat{A}_c$ through the decomposition above such that $\E[\hat{A}_o + \hat{A}_c] = A + o\Para{\frac{1}{n}}$. 
% %$\hfill \square$

Next we show the moment and asymptotical property of $\hat{A}_c$ appeared in \Cref{thm:main}.
%\subsection{Proof of~\Cref{prop:moment}}
Through~\Cref{eq:debias-term}, we have $\E[\hat{A}_c] = \E[\hat{A}_c']+ o\Para{\frac{1}{n}}$.

It is easy to see
\begin{align*}
   \E[\hat{A}_c'] &= -\frac{1}{n^2}\sum_{i = 1}^n \E[\nabla_{\theta} h(\bestx;\xi)^{\top}IF_{\theta^*}(\xi)] \\
   &= -\frac{1}{n}\E[\nabla_{\theta}h(\bestx;\xi)^{\top}IF_{\theta^*}(\xi)] = O\Para{\frac{1}{n}}. 
\end{align*}
Meanwhile, assuming $\E_{\P^*}[\Para{\gradp h(\paranx;\xi)^{\top} IF_{\theta}(\xi)}^2] < \infty$,
%, denote $f(\hat{\theta};\xi) = \nabla_{\theta} h(\datax;\xi_i)^{\top} IF_{\hat{\theta}}(\xi_i)$, 
then:
\begin{align*}
    \E[\hat{A}_{c}^2] &= \frac{1}{n^4}\Para{\sum_{i = 1}^n \E\Paran{\nabla_{\theta} h(\datax;\xi_i)^{\top} IF_{\hat{\theta}}(\xi_i)}}^2\\
    &\leq \frac{1}{n^2}\E\Paran{(\nabla_{\theta} h(\datax;\xi_i)^{\top} IF_{\hat{\theta}}(\xi_i))^2} = O\Para{\frac{1}{n^2}},
\end{align*}
where the inequality follows by $(\sum_{i = 1}^n x_i)^2 \leq n \sum_{i = 1}^n x_i^2$ and the second equality $O\Para{\frac{1}{n^2}}$ follows by the given assumption that $\E_{\P^*}  \Paran{\Para{\nabla_{\theta}h(\paranx;\xi)^{\top} IF_{\theta}(\xi)}^2} < \infty, \forall \theta \in \Theta$. Combining the argument of $\E^2[\hat{A}_c] = O\Para{\frac{1}{n^2}}$, we would then obtain $\var[\hat{A}_c] =\E[\hat{A}_{c}^2] - \E^2[\hat{A}_c]  = O\Para{\frac{1}{n^2}}$.

Finally, we see that:
\begin{align*}
    n \hat{A}_c & = -\frac{1}{n}\sum_{i =1}^n \nabla_{\theta} h(\datax;\xi_i)^{\top} IF_{\hat{\theta}}(\xi_i)\\
    & = - \frac{1}{n}\sum_{i =1}^n \nabla_{\theta} h(\bestx;\xi_i)^{\top} IF_{\theta^*}(\xi_i) + o_p(1)\\
    & \convp -\E[\nabla_{\theta} h(\bestx;\xi)^{\top} IF_{\theta^*}(\xi)],
\end{align*}
where the second equality is trivially from the expectation result in \Cref{eq:oic-unbiased0} and the third line follows by the WLLN. $\hfill \square$
\subsection{Proof of~\Cref{prop:loocv}}
Following the mean-value theorem for each $g_i(\theta) = h(x^*(\theta);\xi_i)$, we have:
\begin{equation}\label{eq:taylor-loocv}
\sum_{i = 1}^n h(x^*(\hat{\theta}_{-i});\xi_i) = \sum_{i = 1}^n h(\datax;\xi_i) + \sum_{i = 1}^n(\hat{\theta}_{-i} - \hat{\theta})^{\top}h(x^*(\tilde{\theta}_{-i});\xi_i),
\end{equation}
where $\tilde{\theta}_{-i}: = \hat{\theta} + a_i (\hat{\theta}_{-i} - \hat{\theta})$ with $|a_i|\leq 1,\forall i \in [n]$.

%Then following~\Cref{asp:theta-asymptotics} and specifc condition, we have:
Besides from conditions in \Cref{prop:loocv}, we have:
\begin{equation}\label{eq:loocv-theta}
    \hat{\theta}_{-i} - \theta^* = - \frac{IF_{\theta^*}(\xi_i)}{n} + o_p\Para{\frac{1}{n}},
\end{equation}
Plugging~\Cref{eq:loocv-theta} back into the second part of right-hand side in~\Cref{eq:taylor-loocv}, we then obtain:
\begin{equation}\label{eq:loocv-final}
    \begin{aligned}
        \sum_{i = 1}^n(\hat{\theta}_{-i} - \hat{\theta})^{\top}h(x^*(\tilde{\theta}_{-i});\xi_i) & = \sum_{i = 1}^n \frac{1}{n (n - 1)}\sum_{j =1, j\neq i}^n IF_{\theta^*}(\xi_j)^{\top}h(x^*(\tilde{\theta}_{-i});\xi_i)\\
        &- \frac{1}{n}\sum_{i = 1}^n IF_{\theta^*}(\xi_i) h(x^*(\tilde{\theta}_{-i});\xi_i) + o_p(1),
    \end{aligned}
\end{equation}
where we can ignore the $o_p(1) = n \times o_p\Para{\frac{1}{n}}$ term since it converges to 0 in probability. We then take an asymptotic view to look at this problem. We observe the following facts from~\Cref{asp:theta-asymptotics}:
\begin{itemize}
    \item $\hat{\theta}_{-i} \convp \theta^*$ as $n \to \infty$ for each $i \in [n]$; It follows simply by observing $\hat{\theta} \convp \theta^*$ as $n \to \infty$.
    \item $\tilde{\theta}_{-i} \convp \hat{\theta}$ since $|a_i|\leq 1$.
\end{itemize}
Following the properties of convergence in probability, we analyze the two terms of right-hand side of~\Cref{eq:loocv-final} respectively.

For the first term from~\Cref{eq:loocv-final}, we have:
\begin{equation*}
\begin{aligned}
    \sum_{i = 1}^n \frac{1}{n (n - 1)}\sum_{j =1, j\neq i}^n IF_{\theta^*}(\xi_j)^{\top}h(x^*(\tilde{\theta}_{-i});\xi_i) &=\frac{1}{n(n- 1)}\sum_{i = 1}^n\sum_{j = 1}^n IF_{\theta^*}(\xi_j)^{\top}h(x^*(\tilde{\theta}_{-i});\xi_i)\\
    &- \sum_{i = 1}^n \frac{1}{n(n - 1)}IF_{\theta^*}(\xi_i)^{\top}h(x^*(\tilde{\theta}_{-i});\xi_i) \\
    &\overset{p}{\to} 0 - 0 = 0,
\end{aligned}
\end{equation*}
where the first term of the third line is base on the fact that $\E_{\P^*}[IF_{\theta^*}(\xi)] = 0$ and therefore, $\frac{1}{n}\sum_{i = 1}^n IF_{\theta^*}(\xi_i)\convp 0$. And the second term of the third line above is given by:
\[\frac{1}{n}\sum_{i = 1}^n IF_{\theta^*}(\xi_i)^{\top} h(x^*(\tilde{\theta}_{-i});\xi_i) \convp \frac{1}{n}\sum_{i = 1}^n IF_{\theta^*}(\xi_i)^{\top} h(x^*(\theta^*);\xi_i) \convp \E_{\P^*}[\nabla_{\theta} h(x^*(\theta);\xi) ^{\top}IF_{\theta^*}(\xi)] < \infty.\]

For the second term from~\Cref{eq:loocv-final}, by WLLN, we have:
\begin{equation*}
    \frac{1}{n}\sum_{i = 1}^n IF_{\theta^*}(\xi_i) h(x^*(\tilde{\theta}_{-i});\xi_i) \convp \frac{1}{n}\sum_{i = 1}^n IF_{\theta^*}(\xi_i) h(\bestx;\xi_i) \convp \E_{\P^*}[\nabla_{\theta} h(x^*(\theta);\xi) ^{\top}IF_{\theta^*}(\xi)].
\end{equation*}
Combining the previous two arguments and plugging into \Cref{eq:loocv-final}, we then obtain:
\[\sum_{i = 1}^n(\hat{\theta}_{-i} - \hat{\theta})^{\top}h(x^*(\tilde{\theta}_{-i});\xi_i) \convp -\E_{\P^*}[\nabla_{\theta} h(x^*(\theta);\xi) ^{\top}IF_{\theta^*}(\xi)].\] 
which is the same as the asymptotics of $n\hat{A}_c$. Furthermore, since $n\hat{A}_o = \sum_{i = 1}^n h(\datax;\xi_i)$, we now show that the estimator obtained from LOOCV is asymptotically equivalent to our proposed estimator in the sense that $n(\hat{A} - \hat{A}_{ocv}) \convp 0$. $\hfill \square$

\subsection{Case of Nonsmooth Objective}\label{app:nonsmooth}
\paragraph{Typical Conditions satisfying \Cref{thm:nonsmooth}.} 
%p20 https://arxiv.org/pdf/1807.02694.pdf
%We borrow some smooth existing results in the nonsmooth objective from literature.
In this nonsmooth case, we assume $Z(\theta) := \E_{\P^*}[h(\paranx;\xi)]$ is twice continuous differentiable near $\theta^*$. Below, we decompose unsmooth in classical objective with compositive function by $h = f(g(\paranx;\xi))$, where $z = g(\paranx;\xi)$ is a smooth function of $\paranx$ and $\xi$ while $f$ may be unsmooth with finite discontinuous points. For example, in the newsvendor problem, $g(\paranx;\xi) = \paranx - \xi, f(z) = c z^+ + (p -c) z^-$, and $h(\paranx;\xi) = f(g(\paranx;\xi))$. 

%For now, we assume $f(\cdot)$ is univariate but the smoothing property can be easily extended to the multivariate case.
We also suppose these $f(z)$ is lower bounded by some constant and locally Lipschitz in the sense that $\forall A > 0$ and $\forall x, y \in [-A, A], |f(x) - f(y)|\leq L_A |x - y|$ with $L_A$ only depending on $A$. Denote $K:= \{z_1,\ldots, z_K\}$ as the set of points where the function $f$ does not have derivatives and $\nabla_u f^-(u) (\nabla_u f^+(u))$ to be the left (right) derivative respectively. 
We give an example of the satisfied sequence of $\{f_m\}$ with the following lemma:
\begin{lemma}[Extracted from \cite{wang2018approximate} under kernel smoothing] \label{lemma:nonsmooth}
Given $\phi(\cdot)$ to be a \textbf{proper kernel} with compact support, and is smooth and symmetric around 0 on $\R$, the smoothed objective function $f_m(z) : = m \int f(u) \phi(m (z - u)) du$ satisfies the following properties:
\begin{enumerate}[(1),leftmargin=*]
    \item $f_m(z) \geq f(z), \forall z \in \R$, and $\lim_{m \to \infty}f_m(z) = f(z), \forall z \in \R$.
    \item $\forall z \in \R \backslash K$, and $\forall m$ large enough, 
    \[\nabla_z f_m(z) = m \int \nabla_u f(u) \phi(m(z-u)) du, \nabla_{zz} f_m(z) = m \int \nabla_{uu}^2 f(u) \phi(m (z-u)) du.\]
    \item $\forall z \in K$, we have:
    \[\lim_{m \to \infty} \nabla_z f_m(z) = \frac{\nabla_z f^-(z) + \nabla_z f^+(z)}{2}, \lim_{m \to \infty} \nabla_{zz}^2 f_m(z) = + \infty.\]
    \item $\lim_{m \to \infty}\E_{z\sim\P}[f_m(z)] = \E_{z\sim \P}[f(z)]$ for any probability distribution $\P$ such that $\E_{z\sim \P}[f(z)] < \infty$.
    %($f_m(z)$ uniformly converges to $f(z)$ under any compact set).
\end{enumerate}
\end{lemma}

Examples of the proper kernel including any box kernel such as $\phi(x) = \frac{1}{2}\mathbf{1}_{\{\|x\|\leq 1\}}$ and epanechnikov kernel $\phi(x) = \frac{3}{4}(1-\|x\|^2)\mathbf{1}_{\{\|x\|\leq 1\}}$. 

\textit{Proof of \Cref{thm:nonsmooth}.}~Under such construction, it is easy to see that $h_m(\paranx;\xi) = f_m(g(\paranx;\xi))$ satisfying $\lim_{m \to \infty}h_m(\paranx;\xi) = h(\paranx;\xi), \forall \xi, \theta$ if we consider $z = g(\paranx;\xi)$ in \Cref{lemma:nonsmooth}(1). Besides, since the second-order derivative of $Z(\theta)$ exists for $\theta$ near $\theta^*$, by definition of derivatives as well as \Cref{lemma:nonsmooth}(4), we also obtain that for any $\theta$ close to $\theta^*$:
\begin{equation}\label{eq:expect}
    \begin{aligned}
        \lim_{m \to \infty}\E_{\P^*}[h_m(\paranx;\xi)] &= \E_{\P^*}[h(\paranx;\xi)].\\
        \lim_{m \to \infty}\nabla_{\theta}\E_{\P^*}[h_m(\paranx;\xi)] &= \nabla_{\theta}\E_{\P^*}[h(\paranx;\xi)].\\
        \lim_{m \to \infty}\hessianp\E_{\P^*}[h_m(\paranx;\xi)] &= \hessianp\E_{\P^*}[h(\paranx;\xi)].\\
    \end{aligned}
\end{equation}

We denote $A_m = \E_{\Dscr^n}\E_{\P^*}[h_m(\datax;\xi)]$. Then for any fixed $m$, we have that OIC for the objective $h_m$, i.e. $\hat{A}_m = \frac{1}{n}\sum_{i = 1}^n h(\datax;\xi_i) - \frac{1}{n^2}\sum_{i = 1}^n\gradp h_m(\datax;\xi_i)^{\top}\hat{IF}_{\hat{\theta}}(\xi_i)$ satisfies $\E[\hat{A}_m] = A_m + o\Para{\frac{1}{n}}$. This follows the same proof structure as in \Cref{thm:main}, i.e. applying the Taylor expansion to $\frac{1}{n}\sum_{i = 1}^n h(\paranx;\xi_i)$ and $\E_{\P^*}[h(\paranx;\xi)]$ at the center $\theta^*$.

Then we observe $\underline{\lim_{m \to \infty}A_m = A + o\Para{\frac{1}{n}}}$ by expanding the function $\E_{\P^*}[h_m(\datax;\xi) - h(\datax;\xi)]$ at the center $\theta^*$ (up to 2nd order with Peano's remainder) such that:
\begin{equation}
    \begin{aligned}
       A_m - A &= \nabla_{\theta}\E_{\P^*}[h_m(\bestx;\xi) - h(\bestx;\xi)]^{\top}\E_{\Dscr^n}[\hat{\theta} - \theta^*]\\
       &+ \frac{1}{2}\E_{\Dscr^n}[(\hat{\theta} - \theta^*)^{\top}\hessianp\E_{\P^*}[h_m(\bestx;\xi) - h(\bestx;\xi)](\hat{\theta} - \theta^*)] + o\Para{\|\hat{\theta} - \theta^*\|^2}. 
    \end{aligned}
\end{equation}
Then we apply \Cref{eq:expect} when $m \to \infty$ and obtain $\lim_{m \to \infty}A_m  = A + o\Para{\frac{1}{n}}$.

On the other hand, from \Cref{eq:expect}, as $m \to \infty$, we can similarly show that:
\[\E\Paran{\frac{1}{n^2}\sum_{i = 1}^n\gradp h_m(\datax;\xi_i)^{\top}\hat{IF}_{\hat{\theta}}(\xi_i) - \frac{1}{n^2}\sum_{i = 1}^n\gradp h(\datax;\xi_i)^{\top}\hat{IF}_{\hat{\theta}}(\xi_i)} = o\Para{\frac{1}{n}},\]
where $\gradp h$ represents the subgradient of $h$ if the function is not differentiable at that point.

Therefore, combining these previous above, 
for $\hat{A}$ in \Cref{eq:oic}, we have:
\[\E[\hat{A}] = \E[\hat{A}_m] + o\Para{\frac{1}{n}} = A_m + o\Para{\frac{1}{n}} = A + o\Para{\frac{1}{n}},\]
which finishes the proof. $\hfill \square$

In practice, for simple, low-dimensional problems, when we can directly evaluate (or approximate) the term $\hessianp \E_{\P^*}[h(\datax;\xi)]$, we do not need to replace it by SAA, e.g., the newsvendor problem demonstrated in \Cref{ex:newsvendor2} and \Cref{app:newsvendor-setup}. For complex objectives, when we cannot simplify $\E_{\P^*}[h(\datax;\xi)]$ to some simple evaluatable form, we can resort to approximate it by $\hessianp\E_{\hat{\P}_n}[h_m(\datax;\xi)]$ where \Cref{lemma:nonsmooth} gives a strategy to evaluate it.
% for appropriately chosen $m$. 

%We discuss the utilities of both approaches for the newsvendor problem in Appendix empirically. 

% Specifically, for the newsvendor, 
% \[h(x;\xi) = c x - p\min\{\xi, x\} = (c - p) x + p \max\{x - \xi, 0\} = \lim_{m \to \infty}\Para{(c - p)x + \frac{p}{m} \log(1 + e^{m(x - \xi)})},\]
% where we denote $h_m(x;\xi) = (c - p)x + \frac{p}{m} \log(1 + e^{m(x - \xi)})$.
The case above does not only work for the nonsmooth objective but can help in the nonsmooth regularizer case. For example, in LASSO Regression, $R(x) = \|x\|_1$, we can approximate with $R_m(x) = \sqrt{\|x\|^2 + \frac{1}{m}}$.

\section{Discussion and Proofs in \Cref{sec:apply}}
\subsection{ETO}
\textit{Proof of \Cref{coro:eto}.}~We plug in the empirical influence function in \Cref{ex:theta-asymptotics} and directly obtain the expression of $\hat{A}_c$. $\hfill \square$

In fact, given the same estimation procedure of $\hat{\theta}$, \Cref{coro:eto} holds as long as the mapping $\theta \mapsto x^*(\theta)$ satisfying \Cref{asp:represent} not restricted to the Problem~\Cref{ex:ddo}(a)(1). For example, \Cref{prop:pf-fit} still holds under the operational statistics approach \citep{liyanage2005practical}, e.g. $\paranx = n[(p/c)^{1/(n + 1)} - 1]\theta$ in \Cref{ex:newsvendor2}. 

%We can incorporate the regularized version in \Cref{subsec:reg} here with the same estimation structure.
\subsection{IEO and E2E}
We list additional assumptions such that \Cref{asp:theta-asymptotics} holds for $\hat{\theta}$ obtained from \Cref{ex:ddo}$(b_1)$, which is classical in the asymptotic analysis.

\begin{assumption}[Conditions of IEO]\label{asp:ierm-additional}
For an open set $\Theta$, suppose that we have:
\begin{enumerate}
    \item Consistency condition: $\sup_{\theta}|\E_{\hat{\P}_n}[h(\paranx;\xi)] - \E_{\P^*}|[h(\paranx;\xi)] \convp 0$; $\forall \epsilon > 0$, $\inf_{\theta \in \Theta, \|\theta - \theta^*\|\geq \epsilon}\E_{\P^*}[h(\paranx;\xi)] > \E_{\P^*}[h(\bestx;\xi)]$.
    \item Regularity condition: For any $\theta_1, \theta_2$ in a neighborhood of $\theta^*$, there exists a measurable function $K$ with $\E_{\P^*}[K^2(\xi)] < \infty$ such that $|h(x^*(\theta_1);\xi) - h(x^*(\theta_2);\xi)| \leq K(\xi)\|\theta_1 - \theta_2\|$. 
    \item Optimality condition: The second order derivative $\hessianp \E_{\P^*}[h(\bestx;\xi)]$ is positive definite.
\end{enumerate}
\end{assumption}

\textit{Proof of \Cref{coro:ierm}.}~Following~\Cref{asp:func}, ~\Cref{asp:ierm-optimality}, we first see by the consistency condition that $\hat{\theta} \convp \theta^*$. Then from \Cref{asp:ierm-additional}, applying results from Theorem 5.23 in \cite{van2000asymptotic} for M-estimators, for the form of influence function in \Cref{asp:theta-asymptotics}, we would attain:
\begin{equation}
    \begin{aligned}
        IF_{\theta^*}(\xi) &= - \Paran{\E_{\P^*}[\hessianp h(\bestx;\xi)]}^{-1}\gradp h(\bestx;\xi),\\
    \end{aligned}
\end{equation}
And the corresponding empirical estimator would be:
\begin{equation}\label{eq:if-ierm}
    \begin{aligned}
         \hat{IF}_{\hat{\theta}}(\xi_i) = -\Paran{\frac{1}{n}\sum_{i = 1}^n\nabla_{\theta\theta}^2 h(\datax;\xi_i)}^{-1} \nabla_{\theta} h(\datax;\xi_i)
    \end{aligned}
\end{equation}    
%For the covariance estimation Error, denote $\hat{A}_{\hat{\theta}} = \E_{\hat{\P}_n}[\hessianp h(\datax;\xi)], \hat{A}_{\theta^*} = \E_{\hat{\P}_n}[\hessianp h(\bestx;\xi)]$, then: $\E_{\Dscr^n}[(\hat{A}_{\hat{\theta}}^{-1} - \hat{A}_{\theta^*}^{-1}) (\hat{A}_{\hat{\theta}}^{-1} - \hat{A}_{\theta^*}^{-1})^{\top}]= o(1)$.
Then we have $\E_{\Dscr^n}[(\hat{IF}_{\hat{\theta}}(\xi) -  IF_{\theta^*}(\xi))(\hat{IF}_{\hat{\theta}}(\xi) - IF_{\theta^*}(\xi))^{\top}] = \E[o(\|\hat{\theta} - \theta^*\|^2)] =o(1)$ by the continuity assumption in \Cref{asp:func} and \Cref{asp:ierm-additional}.

%On the one hand, following LLN, 
% \begin{equation}
%     \begin{aligned}
%         \hat{IF}_{\hat{\theta}}(\xi_i)&= -[\E_{\P^*}[\hessianp h(\bestx;\xi)] + o_p(1)]^{-1}(\gradp h(\bestx;\xi_i) + o_p(1))\\
%         &= IF_{\theta^*}(\xi_i) + o_p(1).
%     \end{aligned}
% \end{equation}
% On the other hand, 
% \begin{equation}
%     \begin{aligned}
%       \E_{\Dscr^n}[\hat{IF}_{\hat{\theta}}(\xi)] &= -\E_{\Dscr^n}\Paran{\Paran{\E_{\P^*}[\hessianp h(\datax;\xi)]}^{-1}\gradp h(\bestx;\xi)} + o(1) \\
%       &= - \Paran{\E_{\P^*}[\hessianp h(\bestx;\xi)]}^{-1}\gradp h(\bestx;\xi) + o(1), 
%     \end{aligned}
% \end{equation}

%where the first equality is implied by Taylor expansion of $\gradp h(\datax;\xi)$ with the center $\gradp h(\bestx;\xi)$ and  by delta method. Therefore, \Cref{asp:if} holds.

Then plugging~\Cref{eq:if-ierm} into $\hat{A}_c$ in~\Cref{thm:main}, since $\hat{A}_c$ is a scale, we would attain:
\begin{equation}
    \begin{aligned}
        \hat{A}_c &= \frac{1}{n^2}\sum_{i = 1}^n \nabla_{\theta} h(\datax;\xi_i)^{\top}\Paran{\frac{1}{n}\sum_{i = 1}^n\nabla_{\theta\theta}^2 h(x^*(\theta);\xi_i)}^{-1} \nabla_{\theta} h(\datax;\xi_i)\\
        & = \text{Tr}\Paran{\frac{1}{n^2}\sum_{i = 1}^n \nabla_{\theta} h(\datax;\xi_i)^{\top}\Paran{\frac{1}{n}\sum_{i = 1}^n\nabla_{\theta\theta}^2 h(x^*(\theta);\xi_i)}^{-1} \nabla_{\theta} h(\datax;\xi_i)}\\
        & = \frac{1}{n}\text{Tr}\Paran{\Paran{\frac{1}{n}\sum_{i = 1}^n\nabla_{\theta\theta}^2 h(\datax;\xi_i)}^{-1}  \frac{1}{n}\sum_{i = 1}^n \nabla_{\theta} h(\datax;\xi_i) \nabla_{\theta} h(\datax;\xi_i)^{\top}},
    \end{aligned}
\end{equation}
where the last equality follows by the fact that $\text{tr}(AB) = \text{tr}(BA)$ and linearity of trace function. $\hfill \square$

We present how \Cref{coro:ierm} demonstrates connections with existing statistic criterion besides AIC.
\begin{example}[Mallow's $C_p$ \citep{mallows2000some}]
Suppose $\xi = (\xi^u, \xi^v)$ with the covariate $\xi^u$ and outcome $\xi^v$, and  $h(x^*(\theta);\xi) = (\xi^v - \theta^{\top}\xi^u)^2$ and therefore this problem aims to minimize MSE based on the regression $\xi^v | \xi^u$. Then $\hat{I}_h(\hat{\theta}) = \frac{2}{n}\sum_{i = 1}^n \xi_{u_i} \xi_{u_i}^{\top} I_{D_{\theta}\times D_{\theta}}$ and $\hat{J}_h(\hat{\theta}) = \frac{1}{n}\sum_{i = 1}^n (\xi_i^v - \theta^{\top} \xi_i^v)(\xi_i^v - \theta^{\top} \xi_i^u)^{\top}$. By simple algebraic manipulation, one can obtain $\hat{A}_c = \frac{2 D_{\theta}\sum_{i = 1}^n (\xi_i^v - \theta^{\top} \xi_i^v)^2}{n^2}$.
\end{example}

% \begin{example}[Stein's unbiased estimator (SURE)]
% [SEE IF WE CAN ADD SURE AS A SPECIAL EXAMPLE.]
% \end{example}
\subsection{$\chi^2$-DRO models}
We state the corresponding influence function for the $f$-divergence DRO problem under the following assumptions.
\begin{assumption}[Conditions of $f$-divergence DRO, extracted from \citep{lam2021impossibility}]\label{asp:dro}
We assume the following holds under the optimization problem~\eqref{eq:dro}.
\begin{enumerate}
    \item \textbf{Lagrangian Multiplier Condition} (related to DRO): $\inf_{\theta \in \Theta} \var_{\P^*}[h(\paranx;\xi)] > 0$; $\forall \theta \in \Theta, \max_{d(\Q, \hat{\P}_n)\leq \epsilon} \E_{\Q}[h(\paranx;\xi)] \neq ess \sup_{\theta}\E_{\hat{\P}_n} h(\paranx;\xi)$. Besides the following optimization problem has a unique solution $(\hat{\theta}, \hat{\alpha}, \hat{\beta})$ satisfying KKT condition with $\hat{\theta}$ in the interior of $\Theta$:
    \[\min_{\theta \in \Theta, \alpha \geq 0, \beta \in R}\Para{\alpha \E_{\hat{\P}_n}\Paran{f^*\Para{\frac{h(\paranx;\xi) - \beta}{\alpha}}}} + \alpha \epsilon + \beta.\]
    \item \textbf{First-order Optimality Condition}: $\theta^*$ is the solution to $\nabla_{\theta}\E_{\P^*}[h(\paranx;\xi)] = 0$ and $\inf_{\theta \in \Theta: \|\theta - \theta^*\|\geq \varepsilon}\|\nabla_{\theta}\E_{\P^*}[h(\paranx;\xi)]\| > 0, \forall \varepsilon > 0$.
    \item \textbf{Regularity Condition}: $h(\paranx;\xi)$ and $\gradp h(\paranx;\xi)$ are uniformly bounded over $\theta \in \Theta$ and $\xi \in \Xi$. And $\|\gradp h(x^*(\theta_1);\xi) - \gradp h(x^*(\theta_2);\xi)\| \leq K(\xi)\|\theta_1 - \theta_2\|$ with $\E_{\P^*}[K^2(\xi)] < \infty$.
    \item \textbf{Function Complexity}: $\{h(\paranx;\cdot), \theta \in \Theta\}, \{h^2(\paranx;\cdot), \theta \in \Theta\}, \{\gradp h(\paranx;\cdot), \theta \in \Theta\}$ are Glivenko-Cantelli. And Donsker property holds for $\{(f^*)'(\alpha h(\paranx;\cdot) - \beta)\gradp h(\paranx;\cdot): 0 \leq \|\theta - \theta^*\|, \alpha,\beta\leq \delta\}$.
\end{enumerate}
\end{assumption}
\begin{lemma}[Extracted from Theorem 4 in \cite{lam2021impossibility}]\label{lemma:dro-if}
Recall the definition of $\hat{\theta}_{\epsilon}$ from~\Cref{eq:dro} and $\theta^* \in \argmin_{\theta}\E_{\P^*}[h(x^*(\theta);\xi)]$. Under Assumption~\ref{asp:func},~\ref{asp:represent} and~\ref{asp:dro}, we have:
\begin{equation*}
\begin{aligned}
    \hat{\theta}_{\epsilon} - \theta^* & = \sum_{i = 1}^n IF_{\theta^*}(\xi_i) - \sqrt{\epsilon (f^{*})''(0)}(\E_{\P^*}[\nabla_{\theta\theta}^2 h(\bestx;\xi)])^{-1}\frac{\cov_p(h(x^*(\theta^*),\xi), \nabla_{\theta}h(x^*(\theta^*),\xi))}{\sqrt{\var_{\P^*}[h(x^*(\theta^*);\xi)]}}\\
    & + o_p\Para{\frac{1}{\sqrt{n}} + \sqrt{\epsilon}},
\end{aligned}
\end{equation*}
where the $IF_{\theta^*}(\xi)$ is the same as that in the empirical optimization.
\end{lemma}
\textit{Proof of~\Cref{coro:dro}.}~The proof is simple as by generalizing $h(x^*;\cdot)$ in \cite{lam2021impossibility} to model-based form $h(x^*(\theta);\cdot)$. Then from \Cref{lemma:dro-if}, denoting the new limiting point of $\hat{\theta}_{\epsilon}$ as:
\[\theta_{\epsilon}^*:= \theta^* - \sqrt{\epsilon (f^{*})''(0)}(\E_{\P^*}[\nabla_{\theta\theta}^2 h(x^*(\theta);\xi)])^{-1}\frac{\cov_p(h(x^*(\theta^*),\xi), \nabla_{\theta}h(x^*(\theta^*),\xi))}{\sqrt{\var_{\P^*}[h(x^*(\theta^*);\xi)]}}.\]
Then consider the asymptotic limit between $\hat{\theta}_{\epsilon}$ and $\theta_{\epsilon}^*$ throughout the proof of~\Cref{thm:main} and~\Cref{coro:ierm}, letting $\epsilon = O\Para{\frac{1}{n}}$, then we have:
\[\hat{\theta}_{\epsilon} - \theta_{\epsilon}^* = \sum_{i = 1}^n IF_{\theta^*}(\xi_i) + o_p\Para{\frac{1}{\sqrt{n}}}.\]
Therefore, we would obtain the same debiasing term as that in~\Cref{coro:ierm}. $\hfill \square$

%\section{Missing Proofs in~\Cref{sec:extension}}

\subsection{Constrained Problem}

\paragraph{Constraints.} We also investigate the following problem with some inequality constraints. Specifically, we consider the following problem:
\begin{equation}\label{eq:constrain-prob}
    \min_{x} \E_{\P^*}[h(x;\xi)]~\text{s.t.}~g_j(x) \leq 0, \forall j \in J.
\end{equation}

We would like the following sets of assumptions to be held for Problem~\eqref{eq:constrain-prob}, which is also prevalent in previous stochastic optimization literature \citep{lam2021impossibility,duchi2021asymptotic}.
\begin{assumption}[Conditions of Constrained Problem]\label{asp:const}
Denote $Z(\theta) = \E_{\P^*}[h(\paranx;\xi)]$, we assume the following under the optimization problem~\eqref{eq:constrain-prob}:
\begin{enumerate}
    \item \textbf{Lagrangian Optimality Condition}: For each $\theta \in \Theta$, the solution $\paranx$ to~\Cref{eq:constrain-prob} solves the problem:
    \[\nabla_{\theta} Z(\theta) + \sum_{j \in B_{\theta}} \alpha_j(\theta) \nabla_{\theta} g_j(x^*(\theta)) = 0,\]
    where $\alpha_j(\theta) > 0$ are the Lagrange multiplers and $B$ indicate the binding active set of constraints. $\{\nabla_{\theta} Z(\theta)\} \cup \{\nabla_{\theta} g_j(x^*(\theta))\}_{j \in B}$ are linearly independent $\forall \theta \in \Theta$. $\alpha_j(\theta), g_j(\paranx)$ is twice differentiable with respect to $\theta$ with $\theta^*$. Besides, the optimal solution $\bestx$, we denote $B$ without subscript to be the corresponding active constraints and $\alpha_j^* = \alpha_j(\theta^*)$.
    Furthermore, $\hessianp Z(\theta^*) + \sum_{j \in B}\alpha_j^* \hessianp g_j(\bestx)$ is positive definite and $\alpha(\theta) g_j(\paranx) = 0, \forall j \in B_{\theta}$.
    \item \textbf{Active Binding Constraints}: The given data-driven solution $\datax$ satisfies $g_j(\datax) = 0, \forall j \in B$ almost surely.
    \item \textbf{Linear Independence Constraint Qualification (LICQ)}: $-Z(\theta^*)$ is the relative interior point of $\{v: v^{\top}(\theta - \theta^*) \leq 0, \forall \theta \in \Theta\}$. 
    \item \textbf{Regularity Condition}: $Z(\paranx)$ is convex in $\theta$. And suppose there exists $C_1 > 0$ such that:
    \[\|\gradp Z(\theta) - \gradp Z(\theta^*)\| \leq C_1 \|\theta - \theta^*\|.\]
    And there exists $C_2, \varepsilon > 0$ such that $\forall \|\theta - \theta^*\| \leq \varepsilon$:
    \[\|\gradp Z(\theta) - \gradp Z(\theta^*) - \hessianp Z(\theta^*)(\theta - \theta^*)\| \leq C_2 \|\theta - \theta^*\|^2.\]
    And there exists $C_3 > 0$ such that $\forall \theta \in \Theta$:
    \[\E_{\P^*}[\|\gradp h(\paranx;\xi) - \gradp h(\bestx;\xi)\|^2] \leq C_3 \|\paranx - \bestx\|^2.\]
    We also assume the empirical multiplier $\hat{\alpha}_j (:= \alpha_j(\hat{\theta})) \overset{a.s.}{\to} \alpha_j^*$.
\end{enumerate}
\end{assumption}

We then attain the following result:
\begin{corollary}\label{coro:constraint}
If Assumption~\ref{asp:func},~\ref{asp:represent},and \ref{asp:const} holds in Problem~\eqref{eq:constrain-prob}, the bias correction term is expressed by:
\[\hat{A}_c =\frac{1}{n}\text{Tr}\Paran{\hat{P} (\hat{I}_{h,\hat{\alpha}}(\hat{\theta}))^{\dagger} \hat{P} \hat{J}(\hat{\theta})}. \]
where $\hat{\alpha}$ is calculated by solving the equation $\nabla_{\theta} Z(\datax) + \sum_{j \in \hat{B}} \hat{\alpha}_j \nabla_{\theta} g_j(\datax) = 0$
with active constraints $\hat{B} = \{j \in J: g_j(\datax) = 0\}$ and $\hat{C} = \{\nabla_{\theta} g_j(\datax)^{\top}\}_{j \in \hat{B}}$, i.e. the matrix whose rows consist of $\nabla_{\theta} g_j(\datax)$ only for the $|\hat{B}|$ active constraints and $\hat{P} = I - \hat{C}(\hat{C}\hat{C})^{\dagger}\hat{C}$ and $ \hat{I}_{h,\alpha}(\hat{\theta}) = \frac{1}{n}\sum_{i = 1}^n \nabla_{\theta\theta}^2 h(\datax;\xi_i) + \sum_{j \in \hat{B}} \hat{\alpha}_j \nabla^2 g_j(\datax)$, where $^{\dagger}$ here denotes the pesudo-inverse.
\end{corollary}
This proof follows the same idea of the standard result with constraint in \Cref{coro:ierm} and the constrained idea in \cite{lam2021impossibility} and Section 2.3 in \cite{duchi2021asymptotic}. Besides the unconstrained case, to compute the estimated influence function, we would also need to estimate the lagrangian multiplers $\hat{\alpha}$ here from the data-driven solution. Compared to the unconstrained result in \Cref{coro:ierm}, the bias correction term becomes smaller by reducing $\hat{I}_{h}(\hat{\theta})$ to $\hat{P}(\hat{I}_{h,\alpha}(\hat{\theta}))\hat{P}$.

%(where $P, I_{h,\alpha}$ is the asymptotic limit of $\hat{P}, \hat{I}_{h,\hat{\alpha}}$ under infinite samples).
% \section{Extension: Nonsmooth function and Contextual Optimization Procedures}\label{sec:extension}
% \subsection{Nonsmooth Results.}\label{subsec:nonsmooth}

%Besides the approximation to the objective, we can do similar things to the regularization term, e.g. $L_1$-regularization to apply the same technique. We leave the full discussion in Appendix.

\textit{Proof of~\Cref{coro:constraint}.}~Since~\Cref{asp:const} holds, we can apply the result of Proposition 1 and Corollary 1 in \cite{duchi2021asymptotic}, where we can illustrate the influence function behavior of $\datax$ under active constraints to be:
\[\hat{\theta} - \theta^* = -P (I_{h,\alpha}(\theta^*))^{\dagger} P\Para{\frac{1}{n}\sum_{i = 1}^n \nabla_{\theta} h(\bestx;\xi_i)} + o_p\Para{\frac{1}{\sqrt{n}}},\]
where if $C \in \R^{|B| \times D_{\theta}}$ denotes the matrix with rows $\{\nabla g_j(\bestx)^{\top}: g_j(\bestx) = 0 \}$, then $P = I - C^{\top}(C C^{\top})^{\dagger} C$, and $I_{h,\alpha}(\theta^*)= \hessianp Z(\bestx) + \sum_{j \in B}\alpha_j^* \hessianp g_j(\bestx)$,
which implies that the influence function for the constrained empirical optimization under this problem would be:
\[IF_{\theta^*}(\xi_i) = -P (I_{h,\alpha}(\theta^*))^{\dagger} P \nabla_{\theta} h(\bestx;\xi_i).\]
Plugging it back into the equation through the proof in~\Cref{thm:main}, we have:
\begin{align*}
    \hat{A}_c^* &=\frac{1}{n^2}\sum_{i = 1}^n \nabla_{\theta} h(\bestx;\xi_i)^{\top}P (I_{h,\alpha}(\theta^*))^{\dagger} P \nabla_{\theta} h(\bestx;\xi_i)\\
    & = \frac{1}{n^2}\text{Tr}\Paran{\sum_{i = 1}^n \nabla_{\theta} h(\bestx;\xi_i)^{\top}P (I_{h,\alpha}(\theta^*))^{\dagger} P \nabla_{\theta} h(\bestx;\xi_i)}\\
    & = \frac{1}{n}\text{Tr}\Paran{P (I_{h,\alpha}(\theta^*))^{\dagger} P \cdot \frac{1}{n}\sum_{i = 1}^n \nabla_{\theta} h(\bestx;\xi_i) \nabla_{\theta} h(\bestx;\xi_i)^{\top}},
\end{align*}
where the second inequality follows the property of the trace. 
Then we can approximate the term $P (I_h(\theta^*))^{\dagger} P$ with $\hat{P} = I - \hat{C}^{\top} (\hat{C}\hat{C}^{\top})^{\dagger}\hat{C}$, and $\hat{I}_{h,\alpha}(\hat{\theta}) = \frac{1}{n}\sum_{i = 1}^n \nabla_{\theta\theta}^2 h(\datax;\xi_i) + \sum_{j \in \hat{B}} \hat{\alpha}_j \nabla^2 g_j(\datax)$ with $\hat{C} = \{\nabla g_j(\datax)^{\top}: g_j(\datax) = 0\}$. From \Cref{asp:const}, we can see that $\hat{P} = P + o_p(1)$ and $P (I_{h,\alpha}(\theta^*))^{\dagger} P  = \hat{P} (\hat{I}_{h,\alpha}(\hat{\theta}))^{\dagger} \hat{P} + o_p(1)$,
such that we can obtain the corresponding $\hat{A}_c = \frac{1}{n}\text{Tr}[\hat{P} (\hat{I}_{h,\alpha}(\hat{\theta}))^{\dagger} \hat{P} \cdot \hat{J}_h(\hat{\theta})]$ with $\hat{J}_h$ the same as the case without constraints. $\hfill \square$

\subsection{Discussion on Contextual Optimization}
\textit{Proof of \Cref{coro:context}.}~For any data-driven solution, we can decompose the true evaluation $A_{con} = \E_{\Dscr^n}\E_z \E_{\P_{\xi|z}^*}[h(x^*(\hat{\theta},z);\xi)]$ to be:
\begin{equation*}
    \begin{aligned}
        A_{con} &= A_{con}' + \E_{z}\E_{\P_{\xi|z}^*}[h(\bestx;\xi_i)] - \frac{1}{n}\sum_{i = 1}^n h(x^*(\theta^*,z_i);\xi_i)\\
    \end{aligned}
\end{equation*}

where $A_{con}' = \E_{\Dscr^n}\E_z \E_{\P_{\xi|z}^*}[h(x^*(\hat{\theta},z);\xi) - h(x^*(\theta^*,z);\xi)] + \frac{1}{n}\sum_{i = 1}^n h(x^*(\theta^*,z_i);\xi_i)$. It is easy to see that:
\begin{equation}\label{eq:unbias-best2}
\begin{aligned}
    &\quad \E\Paran{\frac{1}{n}\sum_{i = 1}^n h(x^*(\theta^*,z_i);\xi_i)} - \E_{z}\E_{\P_{\xi|z}^*}[h(x^*(\theta^*,z);\xi)] \\
    &= \E_{z}\E_{\P_{\xi|z}^*}[h(x^*(\theta^*,z);\xi)] - \E_{z}\E_{\P_{\xi|z}^*}[h(x^*(\theta^*,z);\xi)]  = 0. 
\end{aligned}
\end{equation}
Therefore in order to show $\hat{A}_{con}$ satisfying $\E[\hat{A}_{con}] = A + o\Para{\frac{1}{n}}$, we only need to show that $\hat{A}_{con}$ such that $\E[\hat{A}_{con} - A_{con}'] = o\Para{\frac{1}{n}}$. To see the property of $A_{con}'$, we further notice that:
\begin{equation}
    \begin{aligned}
        A' & = \frac{1}{n}\sum_{i = 1}^n h(x^*(\hat{\theta},z_i);\xi_i) + \underbrace{\frac{1}{n}\sum_{i = 1}^n h(x^*(\theta^*,z_i);\xi_i)  - \frac{1}{n}\sum_{i = 1}^n h(x^*(\hat{\theta},z_i);\xi_i)}_{T_1}\\
&+\underbrace{\E_{\Dscr^n}\E_{\P^*}[h(x^*(\hat{\theta},z);\xi) - h(x^*(\theta^*,z);\xi)]}_{T_2}\\
    \end{aligned}
\end{equation}

The following steps keep the same structure to analyze as that in the proof in \Cref{thm:main}.
$\hfill \square$

Furthermore, in E2E case with the empirical counterpart, given \Cref{asp:ierm-optimality} and \Cref{asp:ierm-additional} while replacing the $x^*(\theta)$ appeared there with $x^*(\theta,z)$, like \Cref{coro:ierm}, the corresponding performance estimator $\hat{A}_{con}$ would be:
\[\hat{A}_{con} = \frac{1}{n}\sum_{i = 1}^n h(x^*(\hat{\theta}, z_i);\xi_i) + \frac{\text{Tr}\Paran{\hat{I}_{h,z}(\hat{\theta})^{-1} \hat{J}_{h,z}(\hat{\theta})}}{n},\]
where the term $\text{Tr}\Paran{\hat{I}_{h,z}(\hat{\theta})^{-1} \hat{J}_{h,z}(\hat{\theta})}$ characterizes the optimistic bias with:
\begin{align*}
    \hat{I}_{h,z}(\hat{\theta})& = \frac{1}{n}\sum_{i = 1}^n \hessianp h(x^*(\hat{\theta},z_i);\xi_i)\\
    \hat{J}_{h,z}(\hat{\theta}) &= \frac{1}{n}\sum_{i = 1}^n \nabla_{\theta}h(x^*(\hat{\theta},z_i);\xi_i) \nabla_{\theta}h(x^*(\hat{\theta},z_i);\xi_i)^{\top}.
\end{align*}

\paragraph{Evaluate Model Mis-specification Error in ETO} Specificially, if we parametrize the model by $\P_{\theta, z}$ and we conduct the estimate-then-optimize procedure, we can obtain a different estimator where the cost function is evaluate under the parametrized distribution like \Cref{prop:pf-fit}. However, we would incur the ``price" of model misspecification. And we can evaluate the ``price" of misspecification similarly in the case in the downstream contextual optimization task, given by the term $B = \E_{\Dscr^n}\E_{\tilde{z}} \E_{\P_{\xi|\tilde{z}}^*}[h(\hat{x};\xi)] - \E_{\Dscr^n}\E_{\P_{\theta^*,\xi|\tilde{z}}}[h(\datax;\xi)]$ through $\hat{B}_{con} = \hat{A}_{con} - \frac{1}{n}\sum_{i = 1}^n A_{z_i}$, where $\hat{A}_{con}$ is defined in~\Cref{eq:context-general} and \begin{equation}\label{eq:context-well}
   \hat{A}_z = \E_{\P_{\hat{\theta}|z}}[h(x^*(\hat{\theta};z);\xi)] + \frac{1}{2n}\text{Tr}[I_{h,z}(\hat{\theta})\Psi(\hat{\theta})] - \frac{\nabla_{\theta}\Para{\E_{\P_{\hat{\theta}}}[h(x^*(\hat{\theta};z);\xi)]}^{\top} C(\P^*, \theta^*)}{n}
\end{equation}
is an estimator of $A_z = \E_{\Dscr^n}\E_{\P^*_{\xi|z}}[h(\hat{x};\xi)]$ with $\E[\hat{A}_z] = A_z + o\Para{\frac{1}{n}}$ (by following the same proof as in \Cref{prop:pf-fit} from \Cref{app:p-oic}). It is easy to see $\E[\hat{B}] = B + o\Para{\frac{1}{n}}$. This provides one procedure to evaluate the model misspecification error in the context optimization side.

% Assuming that we can get access to the solution $x^*(\hat{\theta},z_i)$ for each $z_i$ quickly under the given parametric model. 

% Meanwhile, we can evaluate the effects of the ``best" expected model misspecification error to the downstream optimization problem for the data-driven solution $\hat{x}$ (abbr. of $x^*(\hat{\theta};z)$), i.e.  with:
% \[\hat{B} = \hat{A} - \frac{1}{n}\sum_{i = 1}^n A_{z_i},\]
% such that $\E[\hat{B}] = B + o\Para{\frac{1}{n}}$.
%\subsection{Model-Agnostic Approach}

\subsection{P-OIC: Generalization}\label{app:p-oic}
Here to illustrate~\Cref{prop:pf-fit}, we consider a general case where we express the second-order bias term of order $O\Para{\frac{1}{n}}$ for the estimation of $\hat{\theta}$ than \Cref{asp:theta-asymptotics}.
\begin{assumption}[Statistical Properties of Parameter]\label{asp:theta-asymptotics-strong}
%Denote $\hat{\theta}$ to be the parameter estimated under $\Dscr^n$, 
We have $\hat{\theta}\convp \theta^*$ and:
\[\hat{\theta} - \theta^* = \frac{1}{n}\sum_{i = 1}^n IF_{\theta^*}(\xi_i)  + \frac{C(\P^*, \theta^*)}{n} +  o_p\Para{\frac{1}{\sqrt{n}}}.\]
Additionally, we have: $\sqrt{n}(\hat{\theta} - \theta^*) \convd N(0, \Psi(\theta^*))$, $\E_{\Dscr^n}\Paran{(\hat{\theta} - \theta^*) (\hat{\theta} - \theta^*)^{\top}} = O\Para{\frac{\Psi(\theta^*)}{n}} + o\Para{\frac{1}{n}}$. 
\end{assumption}

Note that if $\hat{\theta}$ is an unbiased estimator of $\theta^*$ then $C(\P^*, \theta^*)$ = 0. 

\begin{example}[Moment methods extracted from \cite{rilstone1996second}]\label{ex:theta-asymptotics-strong}
If the parametric $\hat{\theta}$ and $\theta^*$ is attained from some equation $\E_{\hat{\P}_n}[\psi(\theta;\xi)] = 0$ and $\E_{\P^*}[\psi(\theta;\xi)] = 0$ respectively, then given enough smooth condition for $\psi$ up to third order we would obtain:
\begin{equation}\label{eq:asymptotics-theta}
    \hat{\theta} - \theta^* = a_{-1/2} + a_{-1} +o_p\Para{\frac{1}{n}},
\end{equation}
where $a_{-1/2} = -Q \E_{\hat{\P}_n}[\psi(\theta^*;\xi)] =  O_p(n^{-\frac{1}{2}}),a_{-1} = -Q V a_{-1/2} - \frac{1}{2}Q H [a_{-1/2}\otimes a_{-1/2}] = O_p(n^{-1})$,
and $Q = (\E_{\P^*}[\nabla_{\theta}\psi(\theta^*;\xi))])^{-1}, V = \E_{\P_n}[\nabla_{\theta}\psi(\theta^*;\xi)] - \E_{\P^*}[\nabla_{\theta}\psi(\theta^*;\xi)]$, and $H = \E_{\P^*}[\nabla_{\theta\theta}^2 \psi(\theta^*;\xi))]$, $\otimes$ represents the Kronecker product.
\end{example}
% \begin{assumption}[Optimality Condition]\label{asp:pf-fit-optimal}
% The first-order optimality condition holds for the Problem~\eqref{eq:pf-fit}. Namely, $\bestx$ uniquely solves the equation $\nabla_x \E_{\P_{\theta^*}}[h(x;\xi)] = 0$ and $\datax$ uniquely solves the equation $\nabla_x \E_{\P_{\hat{\theta}}}[h(x;\xi)] = 0$ respectively. Besides, the second order optimality condition holds with $\nabla_{xx}^2 \E_{\P_{\theta^*}}[h(x;\xi)]$ positive definite.
% \end{assumption}

We prove a stronger result indicating the higher-order bias $C(\P^*, \theta^*)$. And it reduces to \Cref{prop:pf-fit} when $\E[\hat{\theta}] = \theta$. That is, $\hat{A}_p = \E_{\P_{\hat{\theta}}}[h(\datax;\xi)] + \frac{1}{2n}\text{Tr}[I_h(\hat{\theta})\Psi(\hat{\theta})]$.
\begin{proposition}[P-OIC]\label{prop:pf-fit-stronger}
If $\P^* = \P_{\theta^*}\in \Pscr_{\Theta}$, and we obtain $\datax$ 
from~\Cref{ex:ddo}(a)(1) and $\nabla_{\theta} \neq 0$. Suppose same conditions in \Cref{thm:main} and optimality condition (\Cref{asp:pf-fit-optimal}) holds, then:
\begin{equation}\label{eq:pf-fit-strong}
    \hat{A}_p = \E_{\P_{\hat{\theta}}}\Paran{h(x^*(\hat{\theta});\xi)} + \frac{1}{2n}\text{Tr}\Paran{I_h(\hat{\theta}) \Psi(\hat{\theta})} - \frac{\nabla_{\theta}\Para{\E_{\P_{\hat{\theta}}}[h(\datax;\xi)]}^{\top} C(\P^*, \theta^*)}{n}
\end{equation}
satisfies $\E[\hat{A}_p] = A + o\Para{\frac{1}{n}}$, where the definition of $I_h(\theta)$ is the same as in~\Cref{coro:ierm}.
\end{proposition}
\textit{Proof of \Cref{prop:pf-fit-stronger}.}Throughout this proof, since we are only considering the decision under the parametric distribution $\P_{\hat{\theta}} (\P_{\theta^*})$, we then $\hat{x} (x^*)$ is abbreviated from $x^*(\hat{\theta}) (x^*(\theta^*))$ respectively.  It is easy to see $\E[\|\hat{x} - x^*\|^2] = O\Para{\frac{1}{n}}$ from \Cref{asp:represent}

%We have the following strategies to construct model selection through nearly unbiased decision quality estimator.

First of all, since the true distribution $\P^*$ is the same as $\P_{\theta^*}$, we can decompose the target term to be:
\begin{equation}\label{eq:param-decomp}
\begin{aligned}
    \E_{\Dscr^n}\E_{\P^*}[h(\hat{x};\xi)]=&\E_{\P_{\hat{\theta}}}[h(\hat{x};\xi)] + \E_{\Dscr^n}\E_{\P_{\hat{\theta}}}\Paran{h(x^*;\xi) - h(\hat{x};\xi)}  \\
    +&\E_{\Dscr^n}\E_{\P^*}\Paran{h(\hat{x};\xi) - h(x^*;\xi)} + \Para{\E_{\P^*}[h(x^*;\xi)] - \E_{\Dscr^n}\E_{\P_{\hat{\theta}}}[h(x^*;\xi)]}
\end{aligned}
\end{equation}

%\underline{(1) Idea 1: [Follow the steps in deriving AIC from KL divergence].} 
In the decomposition above, the second and third term involves the difference between $\hat{x} - x^*$, where the fourth term only evaluates the effects of the estimation error from the distribution to a given quantity. Denote the first term in the right-hand of~\Cref{eq:param-decomp} to be the base estimator, we then can analyze the following term by term.

For the \underline{second term}, by Taylor's expansion up to 2nd with Peano's remainder with the center $x^*$ for the function $u(\theta;\cdot) = \E_{\P_{\theta}}[h(\cdot;\xi)]$, we expand $\E_{\P_{\hat{\theta}}}[h(\hat{x};\xi)]$ as follows:
\begin{equation}
    \begin{aligned}
    \E_{\P_{\hat{\theta}}}[h(x^*;\xi)]& = \E_{\P_{\hat{\theta}}}[h(\hat{x};\xi)] +  \Para{\nabla_{x}\E_{\hat{\theta}}[h(\hat{x};\xi)]}^{\top}(x^* - \hat{x}) + \frac{1}{2}(x^* - \hat{x})^{\top}\Paran{\nabla_{xx}^2\Para{\E_{\hat{\theta}}[h(\hat{x};\xi)]}}(x^* - \hat{x}) + \\
    & + o(\|x^* - \hat{x}\|^2)\\
    & = \E_{\P_{\hat{\theta}}}[h(\hat{x};\xi)] + \frac{1}{2}(x^* - \hat{x})^{\top}\Paran{\nabla_{xx}^2\Para{\E_{\hat{\theta}}[h(x^*;\xi)]}}(x^* - \hat{x}) + o(\|x^* - \hat{x}\|^2),
    \end{aligned}
\end{equation}
%where $\tilde{x} = \hat{x} + a(x^* -\hat{x})$ with $|a|\leq 1$. 
And the second equality follows by applying the first-order condition under the distribution $\P_{\hat{\theta}}$ for the data-driven solution $\hat{x}$ from~\Cref{ex:ddo}(a)(1).
Therefore, taking expectation and we have:
\begin{equation}\label{eq:param-fit-2}
    \E_{\Dscr^n}\E_{\P_{\hat{\theta}}}[h(\hat{x};\xi)] = \E_{\Dscr^n}\E_{\P_{\hat{\theta}}}[h(x^*;\xi)] - \frac{1}{2}\E_{\Dscr^n}\Paran{(\hat{x} - x^*)^{\top} \Para{\nabla_{xx}^2\E_{\P_{\hat{\theta}}}[h(x^*;\xi)]} (\hat{x} - x^*)} + o\Para{\frac{1}{n}}.
\end{equation}

For the \underline{third term}, following the same step and we would obtain:
\begin{equation}\label{eq:param-fit-3}
    \E_{\Dscr^n}\E_{\P^*}[h(\hat{x};\xi))] = \E_{\P^*}[h(x^*;\xi)] + \frac{1}{2}\E\Paran{(\hat{x} - x^*)^{\top} \Para{\nabla_{xx}^2 \E_{\P^*}[h(x^*;\xi)]} (\hat{x} - x^*)} + o\Para{\frac{1}{n}}.
\end{equation}
%where $\tilde{x}' = x^* + b(\hat{x} - x^*)$ with $|b|\leq 1$.
We can further compute $\E\Paran{(\hat{x} - x^*)^{\top} \Para{\nabla_{xx}^2 \E_{\P^*}[h(x^*;\xi)]} (\hat{x} - x^*)} = \frac{1}{n}\text{Tr}[I_h(\theta^*)\Psi(\theta^*)] + o\Para{\frac{1}{n}}$ by algebraic manipulation (i.e. $\gradp^{\top}\bestx \nabla_{xx}^2 \E_{\P^*}[h(x^*;\xi)]\gradp \bestx = \hessianp \E_{\P^*}[h(\bestx;\xi)]$).

For the \underline{fourth term}, denote $u(\theta;x) = \E_{\P_{\theta}}[h(x;\xi)]$, then taking Taylor expansion over $u(\theta;x)$ with respect to $\theta^*$, we have: 
\begin{align*}
   &\quad \E_{\P^*}[h(x^*;\xi)] - \E_{\Dscr^n}\E_{\P_{\hat{\theta}}}[h(x^*;\xi)] \\
   & = u(\theta^*;x^*) - \E_{\hat{\theta}}[u(\hat{\theta};x^*)]\\
   & = -\E_{\Dscr^n}[\hat{\theta} - \theta^*]^{\top} \nabla_{\theta} u(\theta^*;x^*) - \frac{1}{2}\E_{\Dscr^n}[(\hat{\theta} - \theta^*)^{\top} \nabla_{\theta\theta} u(\theta^*;x^*) (\hat{\theta} - \theta^*)] + o\Para{\frac{1}{n}},
\end{align*}
where $\E_{\Dscr^n}[\hat{\theta} - \theta^*] = \frac{C(\P^*, \theta^*)}{n}+ o\Para{\frac{1}{n}}$ from~\Cref{asp:theta-asymptotics-strong}. 
%And $\tilde{\theta} = \theta^* + c(\hat{\theta} - \theta^*)$ for $|c|\leq 1$.

%$|\E_{\P^*}[h(x^*;\xi)] - \E_{\Dscr^n}\E_{\P_{\hat{\theta}}}[h(x^*;\xi)]| \to 0$, 

%TODO: equivalence of xx and \theta\theta
In fact from~\Cref{lemma:matrix-expectation}, one can see that:
\begin{align*}
 \E_{\Dscr^n}[(\hat{\theta} - \theta^*)^{\top} \nabla_{\theta\theta} u(\theta^*;x^*) (\hat{\theta} - \theta^*)] &= \E_{\Dscr^n}\Paran{(\hat{x} - x^*)^{\top}\E_{\P_{\theta^*}}\Paran{\nabla_{xx}^2 h(x^*;\xi)}(\hat{x} - x^*)}\\
 & = \frac{1}{n}\text{Tr}\Paran{I_h(\theta^*)\Psi(\theta^*)} + o\Para{\frac{1}{n}}.
\end{align*}

Combining all the arguments above, we can attain: 
\begin{align*}
    \E_{\Dscr^n}\E_{\P^*}[h(\hat{x};\xi)] &= \E_{\Dscr^n}\E_{\P_{\hat{\theta}}}[h(\hat{x};\xi)] + \E_{\Dscr^n}[(\hat{x} - x^*)^{\top}\nabla_{xx}^2 \E_{\P_{\theta^*}}[h(x^*;\xi)](\hat{x} - x^*)] \\
    & -\frac{1}{2}\E_{\hat{\theta}}[(\hat{\theta} - \theta^*)^{\top} \nabla_{\theta\theta}^2 u(\theta^*;x^*) (\hat{\theta} - \theta^*)]- \nabla_{\theta}\Para{\E_{\P_{\theta^*}}[h(x^*;\xi)]} \frac{C(\P^*, \theta^*)}{n} + o\Para{\frac{1}{n}}\\
    &= \E_{\Dscr^n}\E_{\P_{\hat{\theta}}}[h(\hat{x};\xi)] \\
    & +\frac{1}{2n}\text{Tr}\Paran{I_h(\theta^*)\Psi(\theta^*)}- \nabla_{\theta}\Para{\E_{\P_{\theta^*}}[h(\bestx;\xi)]}^{\top}\frac{C(\P^*, \theta^*)}{n} + o\Para{\frac{1}{n}},
\end{align*}
then replacing $\theta^*$ with $\hat{\theta}$ above, we recover the result of \Cref{prop:pf-fit-stronger}.$\hfill \square$

%Below, we first illustrate the case where the problem is with constraints.

\section{Additional Discussion}

\paragraph{MSE of OIC.} From the main text, we know that the empirical estimator $\hat{A}_o$ would suffer from the bias with $\E[\hat{A}_o]= A + O\Para{\frac{1}{n}}$ while $\hat{A}$ can improve to $\E[\hat{A}_c] = A + o\Para{\frac{1}{n}}$. And we demonstratedthat OIC is still a good decision selection criterion and enjoys similar performance to LOOCV. One pessimistic part is that we cannot improve on the order in terms of $n$ of MSE of decision through OIC. The MSE is computed via:
\begin{equation}
    \begin{aligned}
        \E[A - \hat{A}]^2 &= \E[A - \hat{A}_o - \hat{A}_c]^2 \\
        & = \E[A - \hat{A}_o]^2 + \E[\hat{A}_c^2] - 2 \E[\hat{A}_c (A - \hat{A}_o)]\\
        & \geq \E[A - \hat{A}_o]^2 + O\Para{\frac{1}{n^2}} - 2 \sqrt{\E[\hat{A}_c^2]}\sqrt{\E[(A - \hat{A}_o)^2]}\\
        & = \E[A - \hat{A}_o]^2 + o\Para{\frac{1}{n}},
    \end{aligned}    
\end{equation}
where the equality follows by $\E[(A - \hat{A}_o)^2] = O\Para{\frac{1}{n}}$ and $\E[\hat{A}_c^2] = O\Para{\frac{1}{n^2}}$ from \Cref{thm:main}.

%but it is also not impossible even we are given a set of new samples $\{\xi_i\}_{i \in [n]}$ is independent of the estimated parameter $\hat{\theta}$.
%Denote $A = \E_{\Dscr^n}\E_{\P^*}[h(\hat{x};\xi)]$ as our target estimand and our estimator is $\hat{A}$, which is function of $\Dscr^n$. 
% In previous sections, we establish some $\hat{A}$ such that $\E_{\Dscr^n}[\hat{A}] = A + o\Para{\frac{1}{n}}$. Then we have:
% \begin{align*}
%     \E_{\Dscr^n}\Paran{\hat{A} - A}^2 & = \E\Paran{\hat{A} - \E[\hat{A}]}^2 + \E\Paran{\E[\hat{A}] - A}^2\\
%     & =\Para{\E_{\P^*}[h(x^*;\xi)] - \frac{1}{n}\sum_{i = 1}^n h(x^*;\xi_i)+\ldots}^2 + o\Para{\frac{1}{n^2}} = O\Para{\frac{1}{n}}.
% \end{align*}
In fact, MSE in most of the models (if we use the empirical estimator as the base estimator) would come from $\E_{\P^*}[h(x^*;\xi)] - \frac{1}{n}\sum_{i = 1}^n h(x^*;\xi_i) = O_p\Para{\frac{1}{\sqrt{n}}}$, which is unavoidable and cannot be improved further in terms of the order in $n$ (i.e. Chapter 15 in \cite{wainwright2019high}).
%Sometimes, this fixed estimated error would dominate the potential stochastic error. Therefore, the previous section in debiasing does not help in reducing MSE. On the other hand, confidence intervals for these $A(\hat{x})$ would be dominated by the estimation error above, then the CI is usually not useful to conduct model selection.
Therefore, what we can do is trying to reduce the optimistic bias of each model so that different models can be compared. 

%However, if when we compare across different models in the model selection procedure, this would disappear since each model would face the same set of random samples $\{\xi_1,\ldots, \xi_n\}$ at each time.

\paragraph{Nonparametric Approaches}
We formalize how to apply the bootstrap and jackknife in our problem to derive the corresponding performance estimators $\hat{A}_B, \hat{A}_J$. No matter which method is used, recall $\hat{\theta}$ as the parametric estimator using all the samples $\Dscr^n = \{\xi_i\}_{i = 1}^n$.

%And we give the following debiasing result of the jackknife approach under such case. 
\textbf{Bootstrap.} Denote the bootstrap number as $B_T$. For $b \in [B_T]$, we resample $n$ samples with replacement independently from $\Dscr^n$ as $\{\xi_{b,i}\}_{i \in [n]}$, and compute the corresponding estimator $\hat{\theta}_b$. Then we obtain:
\[\hat{A}_B = 2\hat{A}_o - \frac{1}{B_T}\sum_{b = 1}^{B_T}\hat{A}_{o,b},\]
where $\hat{A}_{o, b} = \frac{1}{n}\sum_{i = 1}^n h(x^*(\hat{\theta}_b);\xi_{b,i}), \forall b \in [B_T]$.

\textbf{Jackknife.} Denote $\hat{\theta}_i$ to be the parametric estimator using samples $\Dscr^n \backslash \{\xi_i\}$. Then we obtain:
\[\hat{A}_J = n \hat{A}_o - \frac{n - 1}{n}\sum_{k = 1}^n A_{o,k},\]
where $\hat{A}_{o,k} = \frac{1}{n - 1}\sum_{i \in [n], i \neq k} h(x^*(\hat{\theta}_k);\xi_i)$.

The following results follow by observing $\E[\hat{A}_o] = A + \frac{\E_{\P^*}[\nabla_{\theta}h(\bestx;\xi)^{\top}IF_{\theta^*}(\xi)]}{n}  + o\Para{\frac{1}{n}}$ from the discussion around \Cref{thm:nonsmooth}.
\begin{lemma}[Debiasing effects, from \cite{quenouille1956notes,hall1994methodology}]\label{lemma:debias}
The bootstrap estimator $\hat{A}_B$ and jackknife estimator $\hat{A}_J$ satisfy: $\E[\hat{A}_{B}] = A + o\Para{\frac{1}{n}}, \E[\hat{A}_{J}] = A + o\Para{\frac{1}{n}}$.
\end{lemma}

\section{Details in Numerical Studies}\label{app:numeric}
Each attribution experiment was run on a cluster using 24 cores from an Intel Xeon Gold 6126 Processor and 16 GB of memory. We use \texttt{cvxpy} with the \texttt{MOSEK} solver to solve the optimization problems in \Cref{subsec:portfolio} and \Cref{subsec:newsvendor}.

%All the codes presented in this paper are available at: \url{https://github.com/wangtianyu61/oic_codes}.

\subsection{Discussion on Influence Functions}
Throughout the two case studies, we consider the moment estimators $\hat{\mu} = \frac{1}{n}\sum_{i = 1}^n \xi_i$ and $\hat{\sigma}^2 =\frac{1}{n}(\xi_i - \hat{\mu})^2$. Then it is easy to see the influence functions of mean, variance estimators from i.i.d. samples, e.g.:
\begin{equation}\label{eq:if-mean-var}
\begin{aligned}
    IF_{\hat{\mu}}(\xi_i) &= \xi_i - \mu \\
    IF_{\hat{\sigma}^2}(\xi_i) & = (\xi_i - \mu)^2 - \sigma^2,
\end{aligned}
\end{equation}
where $\mu = \E[\xi]$ and $\sigma^2 = \var[\xi]$. We can approximate them by the empirical influence functions as:
\begin{equation}\label{eq:eif-mean-var}
\begin{aligned}
    \hat{IF}_{\hat{\mu}}(\xi_i) &= \xi_i - \hat{\mu}\\
    \hat{IF}_{\hat{\sigma}^2}(\xi_i) & = (\xi_i - \hat{\mu})^2 - \hat{\sigma}^2.
\end{aligned}
\end{equation}
We can check $\E[(\hat{IF}_{\hat{\mu}}(\xi) - IF_{\mu}(\xi))^2], \E[(\hat{IF}_{\hat{\sigma}^2}(\xi) - IF_{\sigma^2}(\xi))^2] = o(1)$ as long as $\xi$ has fourth moments. 
%For simplicity, we remove constraints for now and investigate the pure objective performance.

% \subsection{Gradient Evaluation in General Models}

% We use \texttt{torch} to compute the gradients and hessian when it is difficult to manipulate by hand.
    
\subsection{Portfolio Optimization}\label{app:portfolio}
\subsubsection{Detailed Setups}
\textbf{DGP.}~The asset returns $\xi = (\xi_A, \xi_B)^{\top}$ with $\xi_A \sim N(\mu_A,
\Sigma_A)$, $\xi_B \sim N(\mu_B, \Sigma_B)$, $\xi_A \perp \xi_B$, $D_{\xi_A} =
D_{\xi_B} = \frac{1}{2}D_{\xi}$ denoting two classes of assets. For each instance, we generate each entry of $\mu_A, \mu_B \sim U(0, 4)$ and $\Sigma_A, \Sigma_B = CC^{\top}$ while each entry $c_{ij} \sim U(0, \frac{1}{2})$ from $C = \{c_{ij}\}_{i,j \in [D_{\xi_A}]}$. We further denote $A(\xi) = (\xi - \E\xi)(\xi - \E\xi)^{\top}\in \R^{d\times d}$.

We consider the following optimization decision classes:

\textbf{E2E under different policy spaces}. Suppose we have the following E2E with different mappings. 
\underline{SAA-U: Equally Weighted for every asset.} We restrict the space of $\Xscr$ such that the allocation amount to all the assets is the same, i.e., $x^*(\theta) = \theta \mathbf{1}_{D_{\xi}}$ with $\theta \in \R$. Then the space $\Theta = \R$. And plugging in, we have:
$$ h(x^*(\theta);\xi) = (\sum_{i,j}^d A(\xi)_{i,j} + \lambda_2 d)\theta^2 - (\lambda_1 \xi^{\top} \mathbf{1}_d)\theta.$$ 

In this case, $\text{Tr}[I_h(\theta^*)^{-1}J_h(\theta^*)]$ can be expressed (and approximated) by:
\begin{align*}
    \text{Tr}[I_h(\theta^*)^{-1}J_h(\theta^*)] &= \E_{\P^*}\left[\frac{1}{2(\sum_{i,j}^d A(\xi)_{i,j} + \lambda_2 d)}\right] \E_{\P^*}[((\sum_{i,j}^d A(\xi)_{i,j} + \lambda_2 d) 2\theta^* - \lambda_1 \xi^{\top}\mathbf{1}_d)^2]\\
    &\approx \E_{\hat{\P}_n}\left[\frac{1}{2(\sum_{i,j}^d A(\xi)_{i,j} + \lambda_2 d)}\right] \E_{\hat{\P}_n}[((\sum_{i,j}^d A(\xi)_{i,j} + \lambda_2 d) 2\hat{\theta} - \lambda_1 \xi^{\top}\mathbf{1}_d)^2]
\end{align*}

\underline{SAA-B: Block Equally Weighted.} (i.e. equally weighted for assets in one class). This means $\paranx = (\theta_1\mathbf{1}_{D_{\xi_A}}^{\top}, \theta_2 \mathbf{1}_{D_{\xi_B}}^{\top})^{\top}$ with $\theta_1, \theta_2 \in \R$.

\underline{SAA.} That means $x^*(\theta) = \theta \in \Theta$, i.e. the space $\Theta = \R^{D_{\xi}}$. And the bias would be:
\begin{align*}
    \text{Tr}[I_h(\theta^*)^{-1}J_h(\theta^*)] &= \text{Tr}\left(\frac{\E_{\P^*}[(A(\xi) + \lambda_2 I)^{-1}]}{2} \E_{\P^*}[(2(A(\xi) + \lambda_2 I)\theta^* - \lambda_1 \xi)(2(A(\xi) + \lambda_2 I)\theta^* - \lambda_1 \xi)^{\top}]\right)\\
    &\approx \text{Tr}\left(\frac{\E_{\hat{\P}_n}[(A(\xi) + \lambda_2 I)^{-1}]}{2} \E_{\hat{\P}_n}[(2(A(\xi) + \lambda_2 I)\hat{\theta} - \lambda_1 \xi)(2(A(\xi) + \lambda_2 I)\hat{\theta} - \lambda_1 \xi)^{\top}]\right)
\end{align*}

%[TDOO: HOW SAA INVOLVES WITH COMPLEXITY, SHOW IT INCREASES WITH $D_{\xi}^2$]

\textbf{$f$-divergence DRO E2E.} For simplicity, here we only consider DRO models with a specific $f$-divergence, i.e. $\chi^2$-divergence. That is, $f(t) = t^2 - 1$ in $d_f(\P, \Q) = \int f\Para{\frac{d\P}{d\Q}} d\Q$ in \Cref{eq:dro}. We evaluate results with ambiguity levels $\epsilon = \frac{\rho}{n}$ across different $\rho$. Since $h(x;\xi)$ is convex, we can directly apply results in \cite{ben2013robust,duchi2019variance} to obtain convex reformulations for this type of problem and call the standard convex solvers.

\textbf{Parametric Models.} We consider the parametric model class of Gaussian models with independent margins $\P_{\theta} = \{\prod_{i \in [D_{\xi}} N(\mu_i, \sigma_i^2): \theta = (\mu, \sigma)\}$ and apply the ETO approach. Specifically, we plug $\hat{IF}_{\hat{\theta}}(\xi) = (\xi - \hat{\mu}_1,\ldots,\xi - \hat{\mu}_{D_{\xi}}, (\xi - \hat{\mu}_1)^2 - \hat{\sigma}_1,\ldots, (\xi - \hat{\mu}_{D_{\xi}})^2 - \hat{\sigma}_{D_{\xi}}^2)^{\top}$ into the bias term $\hat{A}_c$ via \Cref{coro:eto}.

\paragraph{Evaluation.} For the model bias evaluated in the main text, we compute the true one with: $A - \hat{A}_o$, where $A$ is the true cost of the decision and $\hat{A}_o$ is the empirical cost of the decision,  and bias of other evaluation methods with $A - \hat{A}$ where $\hat{A}$ is the cost of the considered decision.

\subsubsection{Additional Results}
First, we evaluate more data generating setups varying sample size $n$ and $D_{\xi}$ to understand the variation in optimistic bias across different methods in Table~\ref{tab:add-bias1},~\ref{tab:add-bias2} and~\ref{tab:add-bias3}. Due to computational considerations, we only report results of OIC against 2, 5, 10-fold cross validation approaches. From these three tables, we can have consistent observations with those in the main text. OIC can estimate the optimistic bias quite closely to the true bias across all different methods compared with those cross-validation methods. Besides, $\chi^2$-DRO method would incur less bias than the empirical counterpart across different setups. And the intrinsic optimistic bias of ETO method (i.e. Param) under gaussian models with independent margins is quite small.
 
%from the two Figures that no method can outperform OIC.

\begin{table}[htbp]
\centering
\caption{Evaluation of Method Bias with $n = 100, D_{\xi} = 10, \rho = 3$}
\label{tab:add-bias1}
\begin{tabular}{l|ccccc}
\toprule
 & True       & OIC & 2-CV & 5-CV & 10-CV \\
 \midrule
SAA&0.045\scriptsize $\pm 0.030$&0.047\scriptsize $\pm 0.013$&0.078\scriptsize $\pm 0.028$&0.055\scriptsize $\pm 0.017$&0.051\scriptsize $\pm 0.015$\\
SAA-U&0.027\scriptsize $\pm 0.027$&0.023\scriptsize $\pm 0.007$&0.040\scriptsize $\pm 0.018$&0.026\scriptsize $\pm 0.009$&0.025\scriptsize $\pm 0.008$\\
SAA-B&0.039\scriptsize $\pm 0.029$&0.037\scriptsize $\pm 0.011$&0.062\scriptsize $\pm 0.024$&0.043\scriptsize $\pm 0.014$&0.040\scriptsize $\pm 0.012$\\
Param&0.026\scriptsize $\pm 0.056$&0.030\scriptsize $\pm 0.010$&0.018\scriptsize $\pm 0.009$&0.026\scriptsize $\pm 0.007$&0.028\scriptsize $\pm 0.008$\\
DRO&0.044\scriptsize $\pm 0.028$&0.042\scriptsize $\pm 0.011$&0.083\scriptsize $\pm 0.027$&0.055\scriptsize $\pm 0.016$&0.051\scriptsize $\pm 0.014$\\
 \bottomrule
\end{tabular}
\end{table}
 
\begin{table}[htbp]
\centering
\caption{Evaluation of Method Bias with $n = 100, D_{\xi} = 20, \rho = 3$}
\label{tab:add-bias2}
\begin{tabular}{l|ccccc}
\toprule
 & True       & OIC & 2-CV & 5-CV & 10-CV \\
 \midrule
SAA&0.326\scriptsize $\pm 0.108$&0.296\scriptsize $\pm 0.061$&0.561\scriptsize $\pm 0.130$&0.396\scriptsize $\pm 0.091$&0.370\scriptsize $\pm 0.081$\\
SAA-U&0.106\scriptsize $\pm 0.081$&0.113\scriptsize $\pm 0.024$&0.204\scriptsize $\pm 0.058$&0.147\scriptsize $\pm 0.037$&0.139\scriptsize $\pm 0.032$\\
SAA-B&0.178\scriptsize $\pm 0.090$&0.177\scriptsize $\pm 0.038$&0.322\scriptsize $\pm 0.081$&0.231\scriptsize $\pm 0.056$&0.217\scriptsize $\pm 0.051$\\
Param&0.294\scriptsize $\pm 0.562$&0.498\scriptsize $\pm 0.114$&-0.018\scriptsize $\pm 0.196$&0.318\scriptsize $\pm 0.081$&0.402\scriptsize $\pm 0.107$\\
DRO&0.288\scriptsize $\pm 0.090$&0.236\scriptsize $\pm 0.047$&0.483\scriptsize $\pm 0.109$&0.345\scriptsize $\pm 0.077$&0.323\scriptsize $\pm 0.068$\\
 \bottomrule
\end{tabular}
\end{table}

\begin{table}[htbp]
\centering
\caption{Evaluation of Method Bias with $n = 50, D_{\xi} = 20, \rho = 3$}
\label{tab:add-bias3}
\begin{tabular}{l|ccccc}
\toprule
 & True       & OIC & 2-CV & 5-CV & 10-CV \\
 \midrule
SAA&0.168\scriptsize $\pm 0.055$&0.154\scriptsize $\pm 0.027$&0.256\scriptsize $\pm 0.053$&0.187\scriptsize $\pm 0.036$&0.175\scriptsize $\pm 0.034$\\
SAA-U&0.062\scriptsize $\pm 0.048$&0.059\scriptsize $\pm 0.012$&0.090\scriptsize $\pm 0.028$&0.069\scriptsize $\pm 0.015$&0.064\scriptsize $\pm 0.014$\\
SAA-B&0.097\scriptsize $\pm 0.049$&0.092\scriptsize $\pm 0.017$&0.147\scriptsize $\pm 0.037$&0.109\scriptsize $\pm 0.023$&0.102\scriptsize $\pm 0.022$\\
Param&0.211\scriptsize $\pm 0.289$&0.247\scriptsize $\pm 0.055$&-0.081\scriptsize $\pm 0.073$&0.148\scriptsize $\pm 0.038$&0.195\scriptsize $\pm 0.045$\\
DRO&0.151\scriptsize $\pm 0.048$&0.130\scriptsize $\pm 0.022$&0.232\scriptsize $\pm 0.044$&0.170\scriptsize $\pm 0.031$&0.158\scriptsize $\pm 0.029$\\
 \bottomrule
\end{tabular}
\end{table}

In terms of $\chi^2$-DRO method, we report other setups varying sample size $n$ and feature dimension $D_{\xi}$ in terms of the ambiguity level $\epsilon = \frac{\rho}{n}$ in \Cref{fig:app-dro}. We can see across all these scenarios, OIC can identify almost correct regions of the ambiguity level $\rho$ that DRO methods outperform the empirical counterpart to help find a good decision compared with the empirical and robust decisions. 
\begin{figure}
    \centering
    \subfloat[$(n, D_{\xi}) = (50, 30)$]
    {
        \begin{minipage}[t]{0.33\textwidth}
            \centering
            \includegraphics[width = 0.9\textwidth]{figs/portfolio/DRO_50_30.pdf}
        \end{minipage}
    }
    \subfloat[$(n, D_{\xi}) = (100, 20)$]
    {
        \begin{minipage}[t]{0.33\textwidth}
            \centering
            \includegraphics[width = 0.9\textwidth]{figs/portfolio/DRO_100_20.pdf}
        \end{minipage}
    }
    \subfloat[$(n, D_{\xi}) = (100, 40)$]
    {
        \begin{minipage}[t]{0.33\textwidth}
            \centering
            \includegraphics[width = 0.9\textwidth]{figs/portfolio/DRO_100_40.pdf}
        \end{minipage}
    }
    \caption{$\chi^2$-DRO estimated costs varying ambiguity levels $\rho$}
    \label{fig:app-dro}
\end{figure}

% \subsubsection{Other models}
% For $\gamma_0, \gamma_1, \gamma_2 > 0$, we consider the exponential utility function for the portfolio case with
% \[h(x;\xi) =\gamma_0 \exp(-\gamma_1 \xi^{\top}x) + \gamma_2 x^{\top}x.\]
% Under Gaussian models with independent margins, we have:
% \[\E_{\P_{\theta}}[h(x;\xi)] = \exp\Paran{-\gamma_1 \mu^{\top}x + \frac{1}{2}\gamma_1^2\Para{\sum_{i = 1}^d \sigma_i^2 x_i^2}}  + \gamma_2 x^{\top}x.\]

\subsection{Newsvendor Problem}\label{app:newsvendor}
\subsubsection{Detailed Setups}\label{app:newsvendor-setup}
For the single-item newsvendor objective, the standard problem is given by:
\[h(x;\xi) = c x - p \min\{\xi,x\},\]
where $x$ is the order quantity, $\xi$ is the random demand. 
We consider $p = 5, c = 2$ here.

For evaluation, we consider $K$-fold cross validation with $K = 2, 3, 4, 5, 10$ and $K = n$ (LOOCV) in the cross validation model class; We consider the nonparametric bootstrap approach with $B = 10, 50$ and jackknife approach considered in \Cref{sec:discuss}. 

\paragraph{SAA.} For the SAA solution where $x^*(\theta) = \theta$, we can easily compute that $\hessianp \E_{\P^*}[h(x^*(\theta);\xi)] = p f(\theta)$. Denote the c.d.f. of the empirical distribution $\hat{\P}_n$ to be $F_n$, then the classical would be $\hat{\theta} = F_n^{-1}\Para{1 - \frac{c}{p}}$.

In fact the exact solution $x^*$ is the $q$-th quantile of the $\xi$'s distribution with $q: = 1- \frac{c}{p}$, i.e. $\theta^* = F^{-1}\Para{1- \frac{c}{p}}$. On the other hand, given by classical results from M-estimators in \cite{van2000asymptotic}, the $q$-quantile, with the estimator $\hat{\theta}$, then $\sqrt{n}(\hat{\theta} - \theta^*)\overset{d}{\to} N\Para{0, \frac{q(1-q)}{f(\theta^*)^2}}$，where $f(\cdot)$ is the p.d.f. of the random variable $\xi$. Then we estimate the asymptotic variance with $\frac{q(1-q)}{\hat{f}(\hat{\theta})^2}$, where $\hat{f}$ is obtained from the kernel density estimator with guarantee that $\E_{\Dscr^n}[(\hat{f}(\hat{\theta}) - f(\theta^*))^2] =  o(1)$. Then plugging the estimator into \Cref{coro:ierm}, the debiasing term of SAA in the newsvendor problem (\Cref{ex:newsvendor2}) would be:
\[\hat{A}_c = \frac{p q(1 - q)}{n\hat{f}(\hat{\theta})} = \frac{c(p - c)}{np\hat{f}(\hat{\theta})},\]

For the Model Class 2-4, no matter under which parametric distribution class, we estimate mean and variance by $\hat{\mu} = \frac{1}{n}\sum_{i =1}^n \xi_i$, and $\hat{\sigma}^2 = \frac{1}{n - 1}\sum_{i = 1}^n (\xi_i - \hat{\mu})^2$ respectively like \cite{siegel2021profit}. If we know the true distribution $\P^* \in \{\P_{\theta}, \theta \in \Theta\}$, then since the estimators of mean and variance are unbiased, then we can apply the same result P-OIC in \Cref{prop:pf-fit}. The bias correction term with the order $O\Para{\frac{1}{n}}$ of $\hat{A}_c$ in \Cref{prop:pf-fit} is the same as the term in corresponding results in \cite{siegel2021profit}, i.e. Proposition 3 in \cite{siegel2021profit} for Exponential and Exponential-OS models; Proposition 6 in \cite{siegel2021profit} for Normal models. 

However, the expressions above only work when the distribution model is well-specified. In general, when $\P^*$ does not belong to the corresponding parametric class (like in our DGP), the P-OIC estimation procedure may incur the non-diminishing mis-specification error for general cost functions. And we resort to estimate via \Cref{coro:eto}. Specifically, the base estimator $\hat{A}_o = frac{1}{n}\sum_{i = 1}^n h(\hat{x};\xi_i)$. And we calculate the bias correction term for $\hat{A}_c$ in \Cref{thm:main} for each ETO procedure:
\begin{equation}\label{eq:oic-nv}
   \hat{A}_c = -\frac{1}{n^2}\sum_{i = 1}^n \nabla_x h(\datax;\xi_i)\nabla_{\theta} x^*(\hat{\theta})^{\top} \hat{IF}_{\hat{\theta}}(\xi_i). 
\end{equation}
Note that since $\xi$ follows from a continuous distribution, and $\nabla_{x} h(x;\xi_i)$ exists everywhere except $\xi_i$ （we use the associated subgradient from \Cref{thm:nonsmooth}. 
%We then fix $\nabla_x h(x;\xi_i)|_{x = \xi_i} = 0$.
And we plug in the concrete term from the following three ETO models into \Cref{eq:oic-nv}.
\begin{itemize}[leftmargin=*]
    \item \textbf{Normal Distributions}: $\hat{\theta} = (\hat{\mu}, \hat{\sigma}^2)$, and the decision rule would be $x^*(\theta) = \mu + \sqrt{\sigma^2} \Phi^{-1}(1 - \frac{c}{p})$. And $\hat{IF}_{\hat{\theta}}(\xi_i) = (\xi_i - \hat{\mu}, (\xi_i - \hat{\mu})^2 - \hat{\sigma}^2)^{\top}$. 

    %Here the partial derivative denotes the subgradient. We can also approximate with $h_m$

    \item \textbf{Exponential Models}: $\hat{\theta} = \hat{\mu}$, and the decision rule would be $x^*(\theta) = \log (p / c) \hat{\theta}$. And $\hat{IF}_{\hat{\theta}}(\xi_i) = \xi_i - \hat{\mu}$.
    \item \textbf{Exponential Models under Operational Statistics}. Operational statistics apply a different integrated approach for the estimation and optimization pipeline. Here $\hat{\theta} = \hat{\mu}$, the decision rule would be $x^*(\hat{\theta}) = n \Paran{(p / c)^{1/(n + 1)}  - 1 }\hat{\theta}$. And $\hat{IF}_{\hat{\theta}}(\xi^i) = \xi_i - \hat{\mu}$.
\end{itemize}

\subsubsection{Results}
We follow the same data evaluation setups as in \cite{siegel2021profit}, i.e. we run over 100 independent runs to report the model performance as one result and average over 100 independent runs to calculate the associated error comparing with the true performance.

We illustrate the full results in \Cref{fig:newsvendor_normal} and \Cref{fig:newsvendor_exponential} with two different DGPs to evaluate different models under different policies varying sample size $n$. In general, the closer one evaluation criterion is to the zero, the better that evaluation criterion would be.

Across different instances, for existing approaches, it is clear to see that the empirical method would lead to consistent optimistic bias and the bootstrap and jackknife approaches can eliminate that part. And most of $K$-fold cross validation would incur pessimistic bias, which matches the empirical observation in \cite{fushiki2011estimation}. When it comes to the comparison between OIC and these existing approaches, OIC can almost remove the optimistic bias. Although it is true that there are some cross validation approaches that can outperform OIC in some instances (e.g. \Cref{fig:newsvendor_normal} $(o)$ and \Cref{fig:newsvendor_exponential} $(t)$), we can see from all instances from the two Figures that no method can outperform OIC.
\begin{figure}
    \centering
    \subfloat[SAA, $n = 25$]
    {
        \begin{minipage}[t]{0.24\textwidth}
            \centering
            \includegraphics[width = 0.9\textwidth]{figs/nv/nv2_SAA_25_normal.pdf}
        \end{minipage}
    }
    \subfloat[Normal, $n = 25$]
    {
        \begin{minipage}[t]{0.24\textwidth}
            \centering
            \includegraphics[width = 0.9\textwidth]{figs/nv/nv2_Normal_25_normal.pdf}
        \end{minipage}
    }
    \subfloat[Exponential, $n = 25$]
    {
        \begin{minipage}[t]{0.24\textwidth}
            \centering
            \includegraphics[width = 0.9\textwidth]{figs/nv/nv2_Exp_25_normal.pdf}
        \end{minipage}
    }
    \subfloat[Exp-OS, $n = 25$]
    {
        \begin{minipage}[t]{0.24\textwidth}
            \centering
            \includegraphics[width = 0.9\textwidth]{figs/nv/nv2_Exp-OS_25_normal.pdf}
        \end{minipage}
    }
    
    \subfloat[SAA, $n = 50$]
    {
        \begin{minipage}[t]{0.24\textwidth}
            \centering
            \includegraphics[width = 0.9\textwidth]{figs/nv/nv2_SAA_50_normal.pdf}
        \end{minipage}
    }
    \subfloat[Normal, $n = 50$]
    {
        \begin{minipage}[t]{0.24\textwidth}
            \centering
            \includegraphics[width = 0.9\textwidth]{figs/nv/nv2_Normal_50_normal.pdf}
        \end{minipage}
    }
    \subfloat[Exponential, $n = 50$]
    {
        \begin{minipage}[t]{0.24\textwidth}
            \centering
            \includegraphics[width = 0.9\textwidth]{figs/nv/nv2_Exp_50_normal.pdf}
        \end{minipage}
    }
    \subfloat[Exp-OS, $n = 50$]
    {
        \begin{minipage}[t]{0.24\textwidth}
            \centering
            \includegraphics[width = 0.9\textwidth]{figs/nv/nv2_Exp-OS_50_normal.pdf}
        \end{minipage}
    }
    
    \subfloat[SAA, $n = 75$]
    {
        \begin{minipage}[t]{0.24\textwidth}
            \centering
            \includegraphics[width = 0.9\textwidth]{figs/nv/nv2_SAA_75_normal.pdf}
        \end{minipage}
    }
    \subfloat[Normal, $n = 75$]
    {
        \begin{minipage}[t]{0.24\textwidth}
            \centering
            \includegraphics[width = 0.9\textwidth]{figs/nv/nv2_Normal_75_normal.pdf}
        \end{minipage}
    }
    \subfloat[Exponential, $n = 75$]
    {
        \begin{minipage}[t]{0.24\textwidth}
            \centering
            \includegraphics[width = 0.9\textwidth]{figs/nv/nv2_Exp_75_normal.pdf}
        \end{minipage}
    }
    \subfloat[Exp-OS, $n = 75$]
    {
        \begin{minipage}[t]{0.24\textwidth}
            \centering
            \includegraphics[width = 0.9\textwidth]{figs/nv/nv2_Exp-OS_75_normal.pdf}
        \end{minipage}
    }
    
    \subfloat[SAA, $n = 100$]
    {
        \begin{minipage}[t]{0.24\textwidth}
            \centering
            \includegraphics[width = 0.9\textwidth]{figs/nv/nv2_SAA_100_normal.pdf}
        \end{minipage}
    }
    \subfloat[Normal, $n = 100$]
    {
        \begin{minipage}[t]{0.24\textwidth}
            \centering
            \includegraphics[width = 0.9\textwidth]{figs/nv/nv2_Normal_100_normal.pdf}
        \end{minipage}
    }
    \subfloat[Exponential, $n = 100$]
    {
        \begin{minipage}[t]{0.24\textwidth}
            \centering
            \includegraphics[width = 0.9\textwidth]{figs/nv/nv2_Exp_100_normal.pdf}
        \end{minipage}
    }
    \subfloat[Exp-OS, $n = 100$]
    {
        \begin{minipage}[t]{0.24\textwidth}
            \centering
            \includegraphics[width = 0.9\textwidth]{figs/nv/nv2_Exp-OS_100_normal.pdf}
        \end{minipage}
    }
    
    \subfloat[SAA, $n = 125$]
    {
        \begin{minipage}[t]{0.24\textwidth}
            \centering
            \includegraphics[width = 0.9\textwidth]{figs/nv/nv2_SAA_125_normal.pdf}
        \end{minipage}
    }
    \subfloat[Normal, $n = 125$]
    {
        \begin{minipage}[t]{0.24\textwidth}
            \centering
            \includegraphics[width = 0.9\textwidth]{figs/nv/nv2_Normal_125_normal.pdf}
        \end{minipage}
    }
    \subfloat[Exponential, $n = 125$]
    {
        \begin{minipage}[t]{0.24\textwidth}
            \centering
            \includegraphics[width = 0.9\textwidth]{figs/nv/nv2_Exp_125_normal.pdf}
        \end{minipage}
    }
    \subfloat[Exp-OS, $n = 125$]
    {
        \begin{minipage}[t]{0.24\textwidth}
            \centering
            \includegraphics[width = 0.9\textwidth]{figs/nv/nv2_Exp-OS_125_normal.pdf}
        \end{minipage}
    }
    \caption{Evaluation results of different Data-Driven solutions under normal-based distributions}
    \label{fig:newsvendor_normal}
\end{figure}

\begin{figure}
    \centering
    \subfloat[SAA, $n = 25$]
    {
        \begin{minipage}[t]{0.24\textwidth}
            \centering
            \includegraphics[width = 0.9\textwidth]{figs/nv/nv2_SAA_25_exponential.pdf}
        \end{minipage}
    }
    \subfloat[Normal, $n = 25$]
    {
        \begin{minipage}[t]{0.24\textwidth}
            \centering
            \includegraphics[width = 0.9\textwidth]{figs/nv/nv2_Normal_25_exponential.pdf}
        \end{minipage}
    }
    \subfloat[Exponential, $n = 25$]
    {
        \begin{minipage}[t]{0.24\textwidth}
            \centering
            \includegraphics[width = 0.9\textwidth]{figs/nv/nv2_Exp_25_exponential.pdf}
        \end{minipage}
    }
    \subfloat[Exp-OS, $n = 25$]
    {
        \begin{minipage}[t]{0.24\textwidth}
            \centering
            \includegraphics[width = 0.9\textwidth]{figs/nv/nv2_Exp-OS_25_exponential.pdf}
        \end{minipage}
    }
    
    \subfloat[SAA, $n = 50$]
    {
        \begin{minipage}[t]{0.24\textwidth}
            \centering
            \includegraphics[width = 0.9\textwidth]{figs/nv/nv2_SAA_50_exponential.pdf}
        \end{minipage}
    }
    \subfloat[Normal, $n = 50$]
    {
        \begin{minipage}[t]{0.24\textwidth}
            \centering
            \includegraphics[width = 0.9\textwidth]{figs/nv/nv2_Normal_50_exponential.pdf}
        \end{minipage}
    }
    \subfloat[Exponential, $n = 50$]
    {
        \begin{minipage}[t]{0.24\textwidth}
            \centering
            \includegraphics[width = 0.9\textwidth]{figs/nv/nv2_Exp_50_exponential.pdf}
        \end{minipage}
    }
    \subfloat[Exp-OS, $n = 50$]
    {
        \begin{minipage}[t]{0.24\textwidth}
            \centering
            \includegraphics[width = 0.9\textwidth]{figs/nv/nv2_Exp-OS_50_exponential.pdf}
        \end{minipage}
    }
    
    \subfloat[SAA, $n = 75$]
    {
        \begin{minipage}[t]{0.24\textwidth}
            \centering
            \includegraphics[width = 0.9\textwidth]{figs/nv/nv2_SAA_75_exponential.pdf}
        \end{minipage}
    }
    \subfloat[Normal, $n = 75$]
    {
        \begin{minipage}[t]{0.24\textwidth}
            \centering
            \includegraphics[width = 0.9\textwidth]{figs/nv/nv2_Normal_75_exponential.pdf}
        \end{minipage}
    }
    \subfloat[Exponential, $n = 75$]
    {
        \begin{minipage}[t]{0.24\textwidth}
            \centering
            \includegraphics[width = 0.9\textwidth]{figs/nv/nv2_Exp_75_exponential.pdf}
        \end{minipage}
    }
    \subfloat[Exp-OS, $n = 75$]
    {
        \begin{minipage}[t]{0.24\textwidth}
            \centering
            \includegraphics[width = 0.9\textwidth]{figs/nv/nv2_Exp-OS_75_exponential.pdf}
        \end{minipage}
    }
    
    \subfloat[SAA, $n = 100$]
    {
        \begin{minipage}[t]{0.24\textwidth}
            \centering
            \includegraphics[width = 0.9\textwidth]{figs/nv/nv2_SAA_100_exponential.pdf}
        \end{minipage}
    }
    \subfloat[Normal, $n = 100$]
    {
        \begin{minipage}[t]{0.24\textwidth}
            \centering
            \includegraphics[width = 0.9\textwidth]{figs/nv/nv2_Normal_100_exponential.pdf}
        \end{minipage}
    }
    \subfloat[Exponential, $n = 100$]
    {
        \begin{minipage}[t]{0.24\textwidth}
            \centering
            \includegraphics[width = 0.9\textwidth]{figs/nv/nv2_Exp_100_exponential.pdf}
        \end{minipage}
    }
    \subfloat[Exp-OS, $n = 100$]
    {
        \begin{minipage}[t]{0.24\textwidth}
            \centering
            \includegraphics[width = 0.9\textwidth]{figs/nv/nv2_Exp-OS_100_exponential.pdf}
        \end{minipage}
    }

    \subfloat[SAA, $n = 125$]
    {
        \begin{minipage}[t]{0.24\textwidth}
            \centering
            \includegraphics[width = 0.9\textwidth]{figs/nv/nv2_SAA_125_exponential.pdf}
        \end{minipage}
    }
    \subfloat[Normal, $n = 125$]
    {
        \begin{minipage}[t]{0.24\textwidth}
            \centering
            \includegraphics[width = 0.9\textwidth]{figs/nv/nv2_Normal_125_exponential.pdf}
        \end{minipage}
    }
    \subfloat[Exponential, $n = 125$]
    {
        \begin{minipage}[t]{0.24\textwidth}
            \centering
            \includegraphics[width = 0.9\textwidth]{figs/nv/nv2_Exp_125_exponential.pdf}
        \end{minipage}
    }
    \subfloat[Exp-OS, $n = 125$]
    {
        \begin{minipage}[t]{0.24\textwidth}
            \centering
            \includegraphics[width = 0.9\textwidth]{figs/nv/nv2_Exp-OS_125_exponential.pdf}
        \end{minipage}
    }
    \caption{Evaluation results of different Data-Driven solutions under exponential-based distributions}
    \label{fig:newsvendor_exponential}
\end{figure}

We also report the decision selection quality under different DGPs. Intuitively, when the underlying true distribution is fully parametric, the corresponding well-specified ETO approach would dominate others \citep{elmachtoub2023estimatethenoptimize} but it is not clear whether SAA or the corresponding parametric approach would be better under mis-specified case. And we do not know how the decision selected by different criterion (including EM, OIC, $K$-fold CV) would behave. We run the same experiment and compare the performance of four models per instance. For each evaluation criterion (e.g. true, empirical costs, OIC costs, costs computed via 5-CV, 10-CV), we choose the one from the four models with smallest cost given the associate criterion. In \Cref{tab:nv-decision-quality}, we find the decision selection given by OIC almost matches the best that we can achieve (close to the true performance) under these four DGPs and strictly dominates the performance of the EM approach.
\begin{table}
\centering
\caption{Decision Quality}
\label{tab:nv-decision-quality}
\begin{tabular}{l|cccccc}
\toprule
     DGP          & True & EM & OIC & 5-CV & 10-CV & LOOCV\\
\midrule
50-normal&-221.72\scriptsize $\pm 0.11$&-221.35\scriptsize $\pm 0.14$&-221.72\scriptsize $\pm 0.11$&-221.71\scriptsize $\pm 0.12$&-221.71\scriptsize $\pm 0.12$&-221.70\scriptsize $\pm 0.14$\\
50-exp.&-115.02\scriptsize $\pm 0.21$&-113.86\scriptsize $\pm 0.47$&-114.99\scriptsize $\pm 0.25$&-114.99\scriptsize $\pm 0.24$&-115.01\scriptsize $\pm 0.21$&-115.01\scriptsize $\pm 0.21$\\
100-normal&-222.14\scriptsize $\pm 0.07$&-221.98\scriptsize $\pm 0.11$&-222.14\scriptsize $\pm 0.07$&-222.14\scriptsize $\pm 0.07$&-222.14\scriptsize $\pm 0.07$&-222.12\scriptsize $\pm 0.10$\\
100-exp.&-115.84\scriptsize $\pm 0.13$&-115.22\scriptsize $\pm 0.23$&-115.82\scriptsize $\pm 0.12$&-115.83\scriptsize $\pm 0.14$&-115.82\scriptsize $\pm 0.16$&-115.79\scriptsize $\pm 0.18$\\
\bottomrule
\end{tabular}
\end{table}

And we ompare the model misspecification error of different ETO models in \Cref{fig:main_nv}(c).

\subsection{Regression Tasks}
\paragraph{Models.}We consider Linear and Ridge regression with 2-polynomial features with $\alpha = 0, 1, 5$, which are default in the \texttt{sklearn.linear\_model.LinearRegression} and  \texttt{sklearn.linear\_model.ridge} module (with polynomial features generated from \texttt{sklearn.preprocessing.PolynomialFeature}). The empirical influence function of $\hat{\theta}$ in those models are computed Suppose the linear regression case with $\xi^v = \theta^{\top} \xi^u + \epsilon$, the empirical influence function of $\hat{\theta}$ under OLS would be:
\begin{equation}\label{eq:if-lr}
\begin{aligned}
    \hat{IF}_{\hat{\theta}}(\xi_i) & = (\xi_i^v - \hat{\theta}^{\top} \xi_i^u) \hat{\Sigma}^{-1}\xi_i^u,
\end{aligned}
\end{equation}
where $\hat{\Sigma} = \frac{1}{n}\sum_{i = 1}^n \xi_i^u (\xi_i^u) ^{\top}$.

In terms of the neural net, we just apply a two-hidden-layer architecture, one with 8 hidden neurons and use \texttt{nn.Softplus()} as the activation unit of each layer, totally 185 parameters. We consider the model with learning rate to be 0.1, batch size to be 128 during the training procedure. We use \texttt{torch.gradient} and \texttt{torch.hessian} to compute gradients and hessians in the neural nets and compute the empirical influence function under the same formulation as that in \Cref{ex:motivating} and \cite{koh2017understanding}. However, the problem in \cite{koh2017understanding} is that the influence function cannot be estimated accurately usually because modern neural networks satisfy these first and second-order optimality conditions at the end of training rarely. Due to this, further refinement in neural networks are proposed in \cite{yeh2018representer,pruthi2020estimating}. We leave better representations in the quality of estimators in these deep models as future work.

%When the neural network is deep with large model parameters, the OIC is computed in the degenerate case by only taking into account the eigenvalues of the Hessian of significant magnitude while cutting all eigenvalues smaller than one threshold.

\paragraph{Evaluation Setups.} In terms of the random seeds, we randomly select 10\% and 30\% of all samples but stratify over red and white wine since the two kinds of wine appear to be quite different, demonstrated in \cite{duchi2023distributionally}.

The evaluation performance of EM, OIC, 5-CV is calculated the same as before since we only need in-sample data. However, we do not know the true performance in this real-world dataset. Therefore, we approximate the true model (oracle) performance $A$ via the out-of-sample performance. In terms of the total sample size $n = n_{tr} + n_{te}$ in each case (where $n_{tr} = 0.1 n$ or $n_{tr} = 0.3n$ for different cases), we use $\{\xi_j\}_{j \in [n_{tr}}$ to train each model (in-sample data) and $\{\xi_{j + n_{tr}}\}_{j \in [n_{te}]}$ to evaluate the true performance approximately. That is to say, for each model $x^*(\hat{\theta}_k)$, we approximate the true model performance $A \approx \frac{1}{n}\sum_{j \in [n_{te}]}h(x^*(\hat{\theta}_k);\xi_{j + n_{tr}})$.

%we approximate the Oracle Performance by out-of-sample performance
%Therefore, the size of different models are:

% \begin{center}
% \begin{tabular}{c|c|c|c}
%     Linear & Quadratic & NN-1 &NN-2 \\
%     \hline
%      & & &
% \end{tabular}
% \end{center}
